# Supplementary material for: Flash STU: Fast Spectral Transform Units
Source: arXiv:2409.10489 source file (2026-01-17)
Supplement: Supplementary file 1 [file appendix_loss_landscape.tex]

\section{Loss Landscapes on Robotics Data}

\begin{figure}[ht]
\centering
% First row
\begin{subfigure}{0.23\textwidth}
    \includegraphics[width=\linewidth]{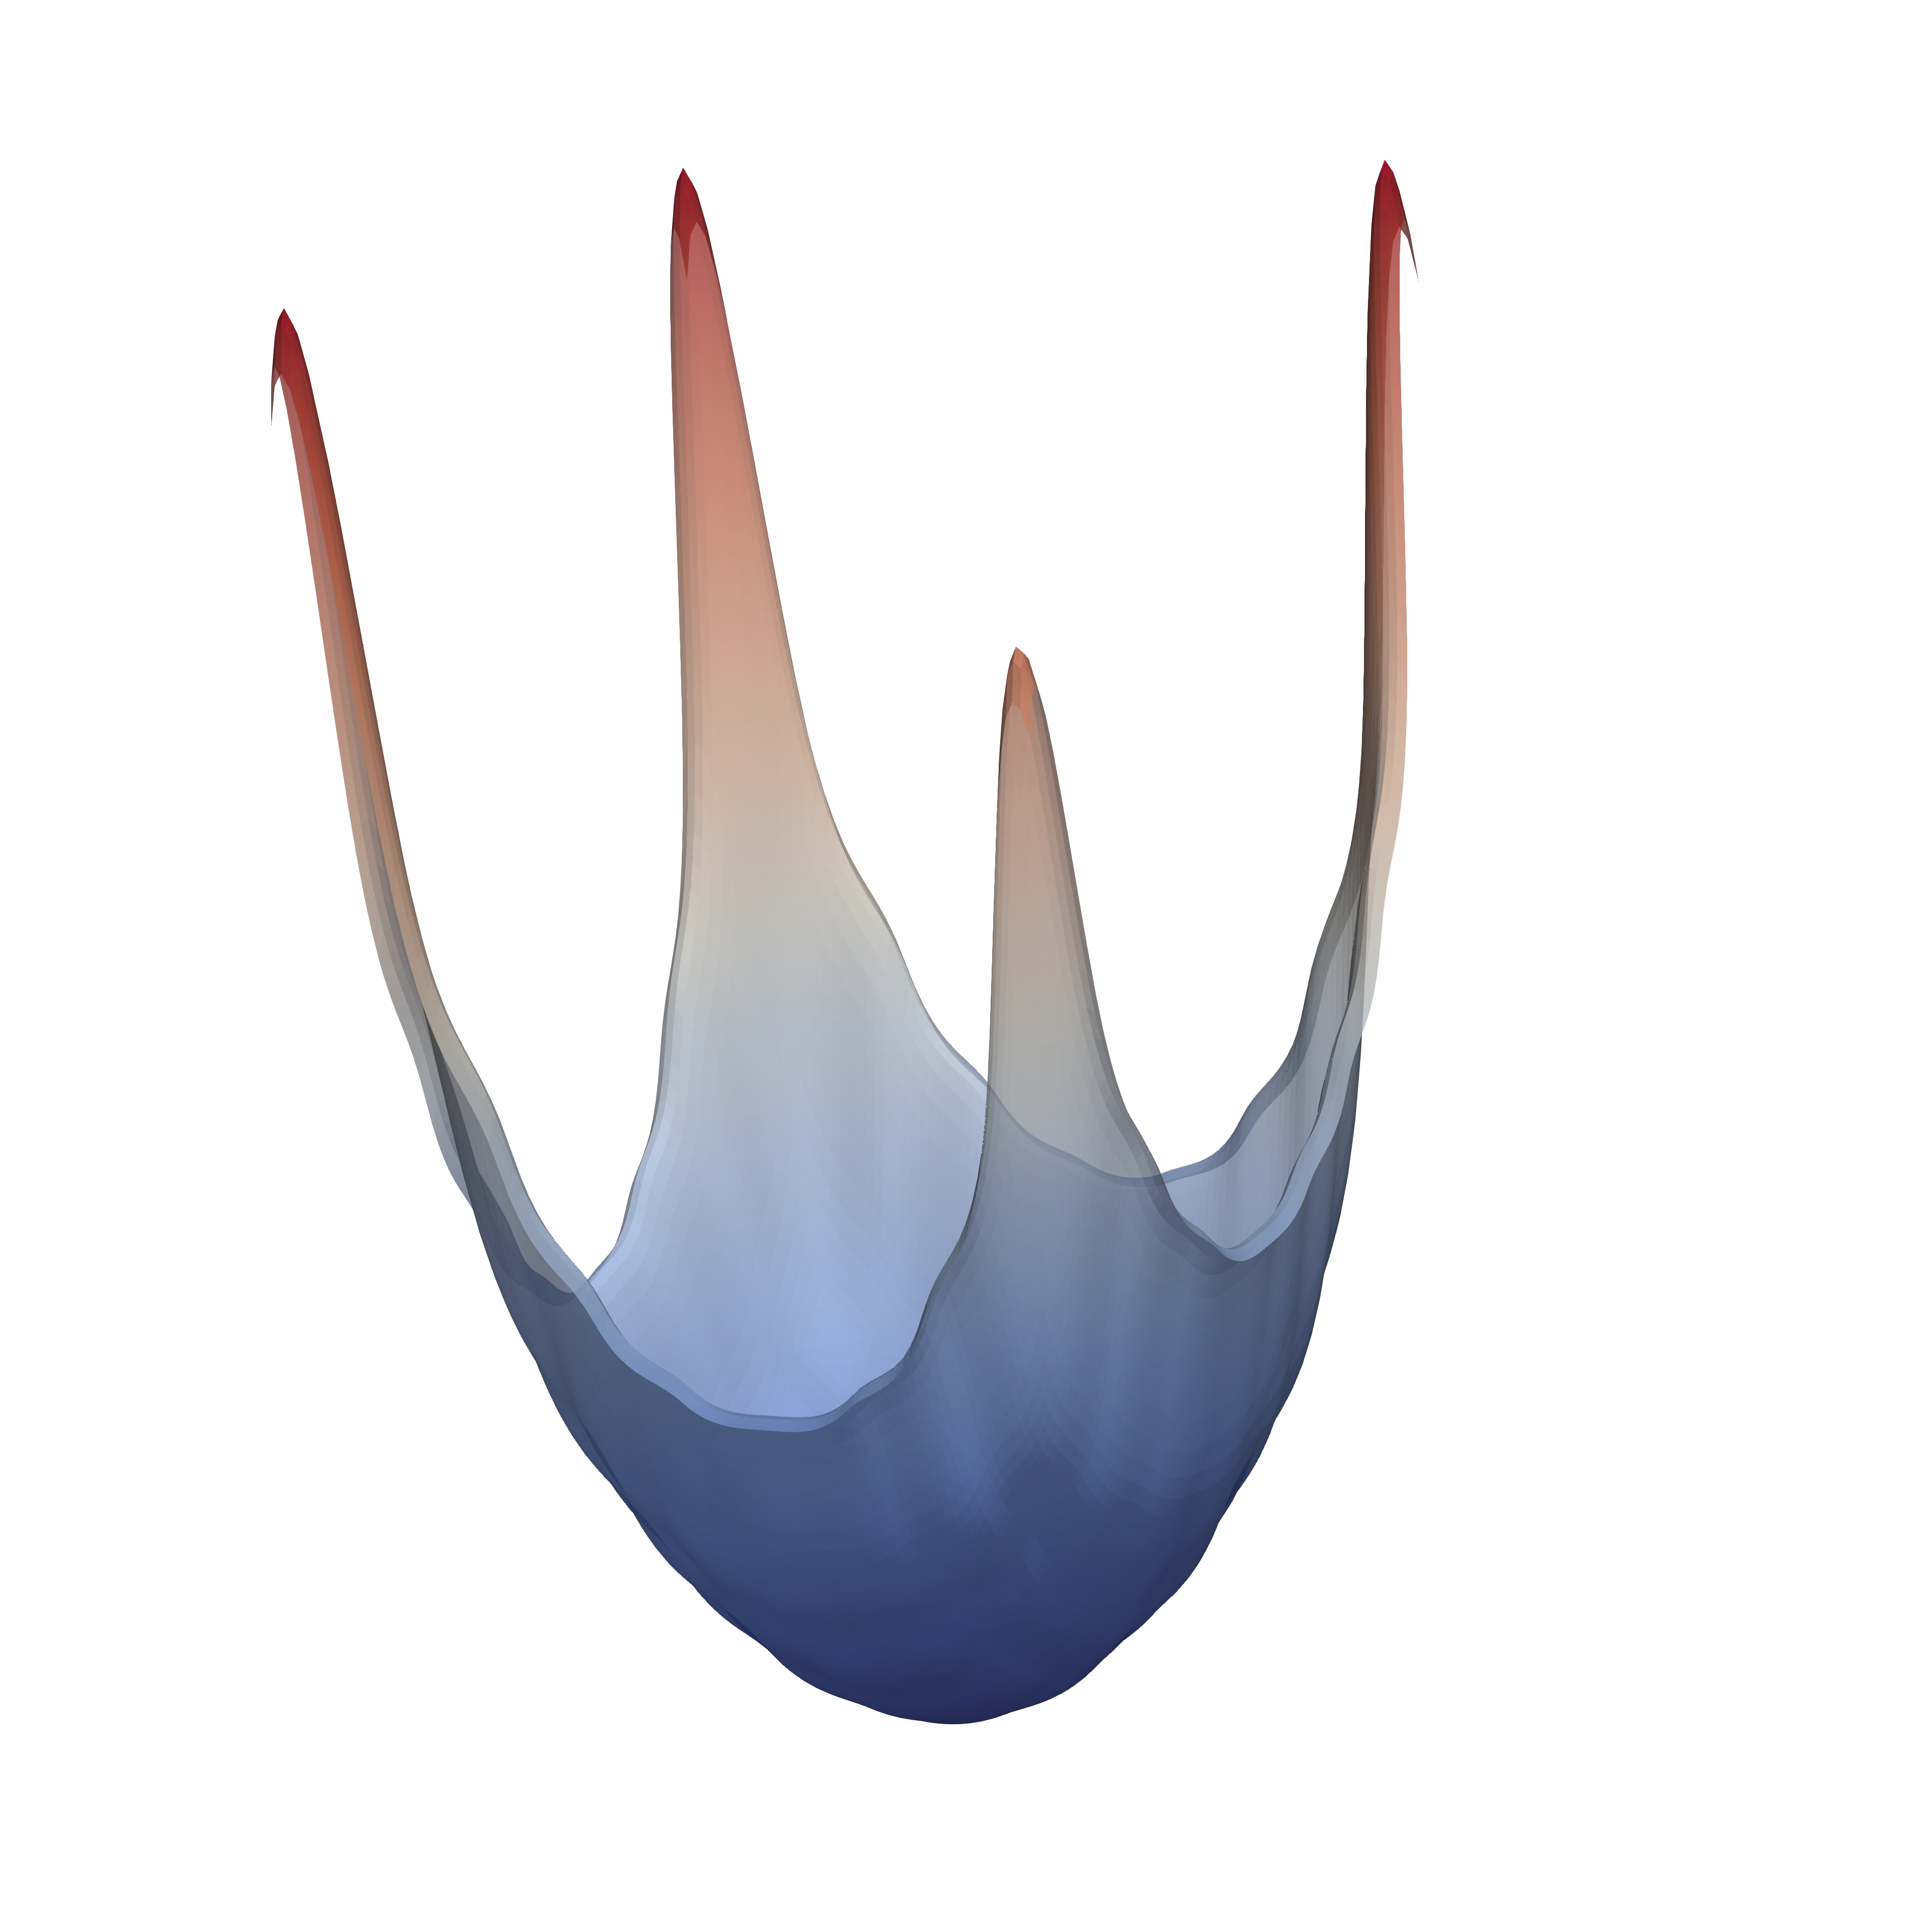}
    \caption{Model Width: 32}
    \label{fig:Transformer32}
\end{subfigure}
\begin{subfigure}{0.23\textwidth}
    \includegraphics[width=\linewidth]{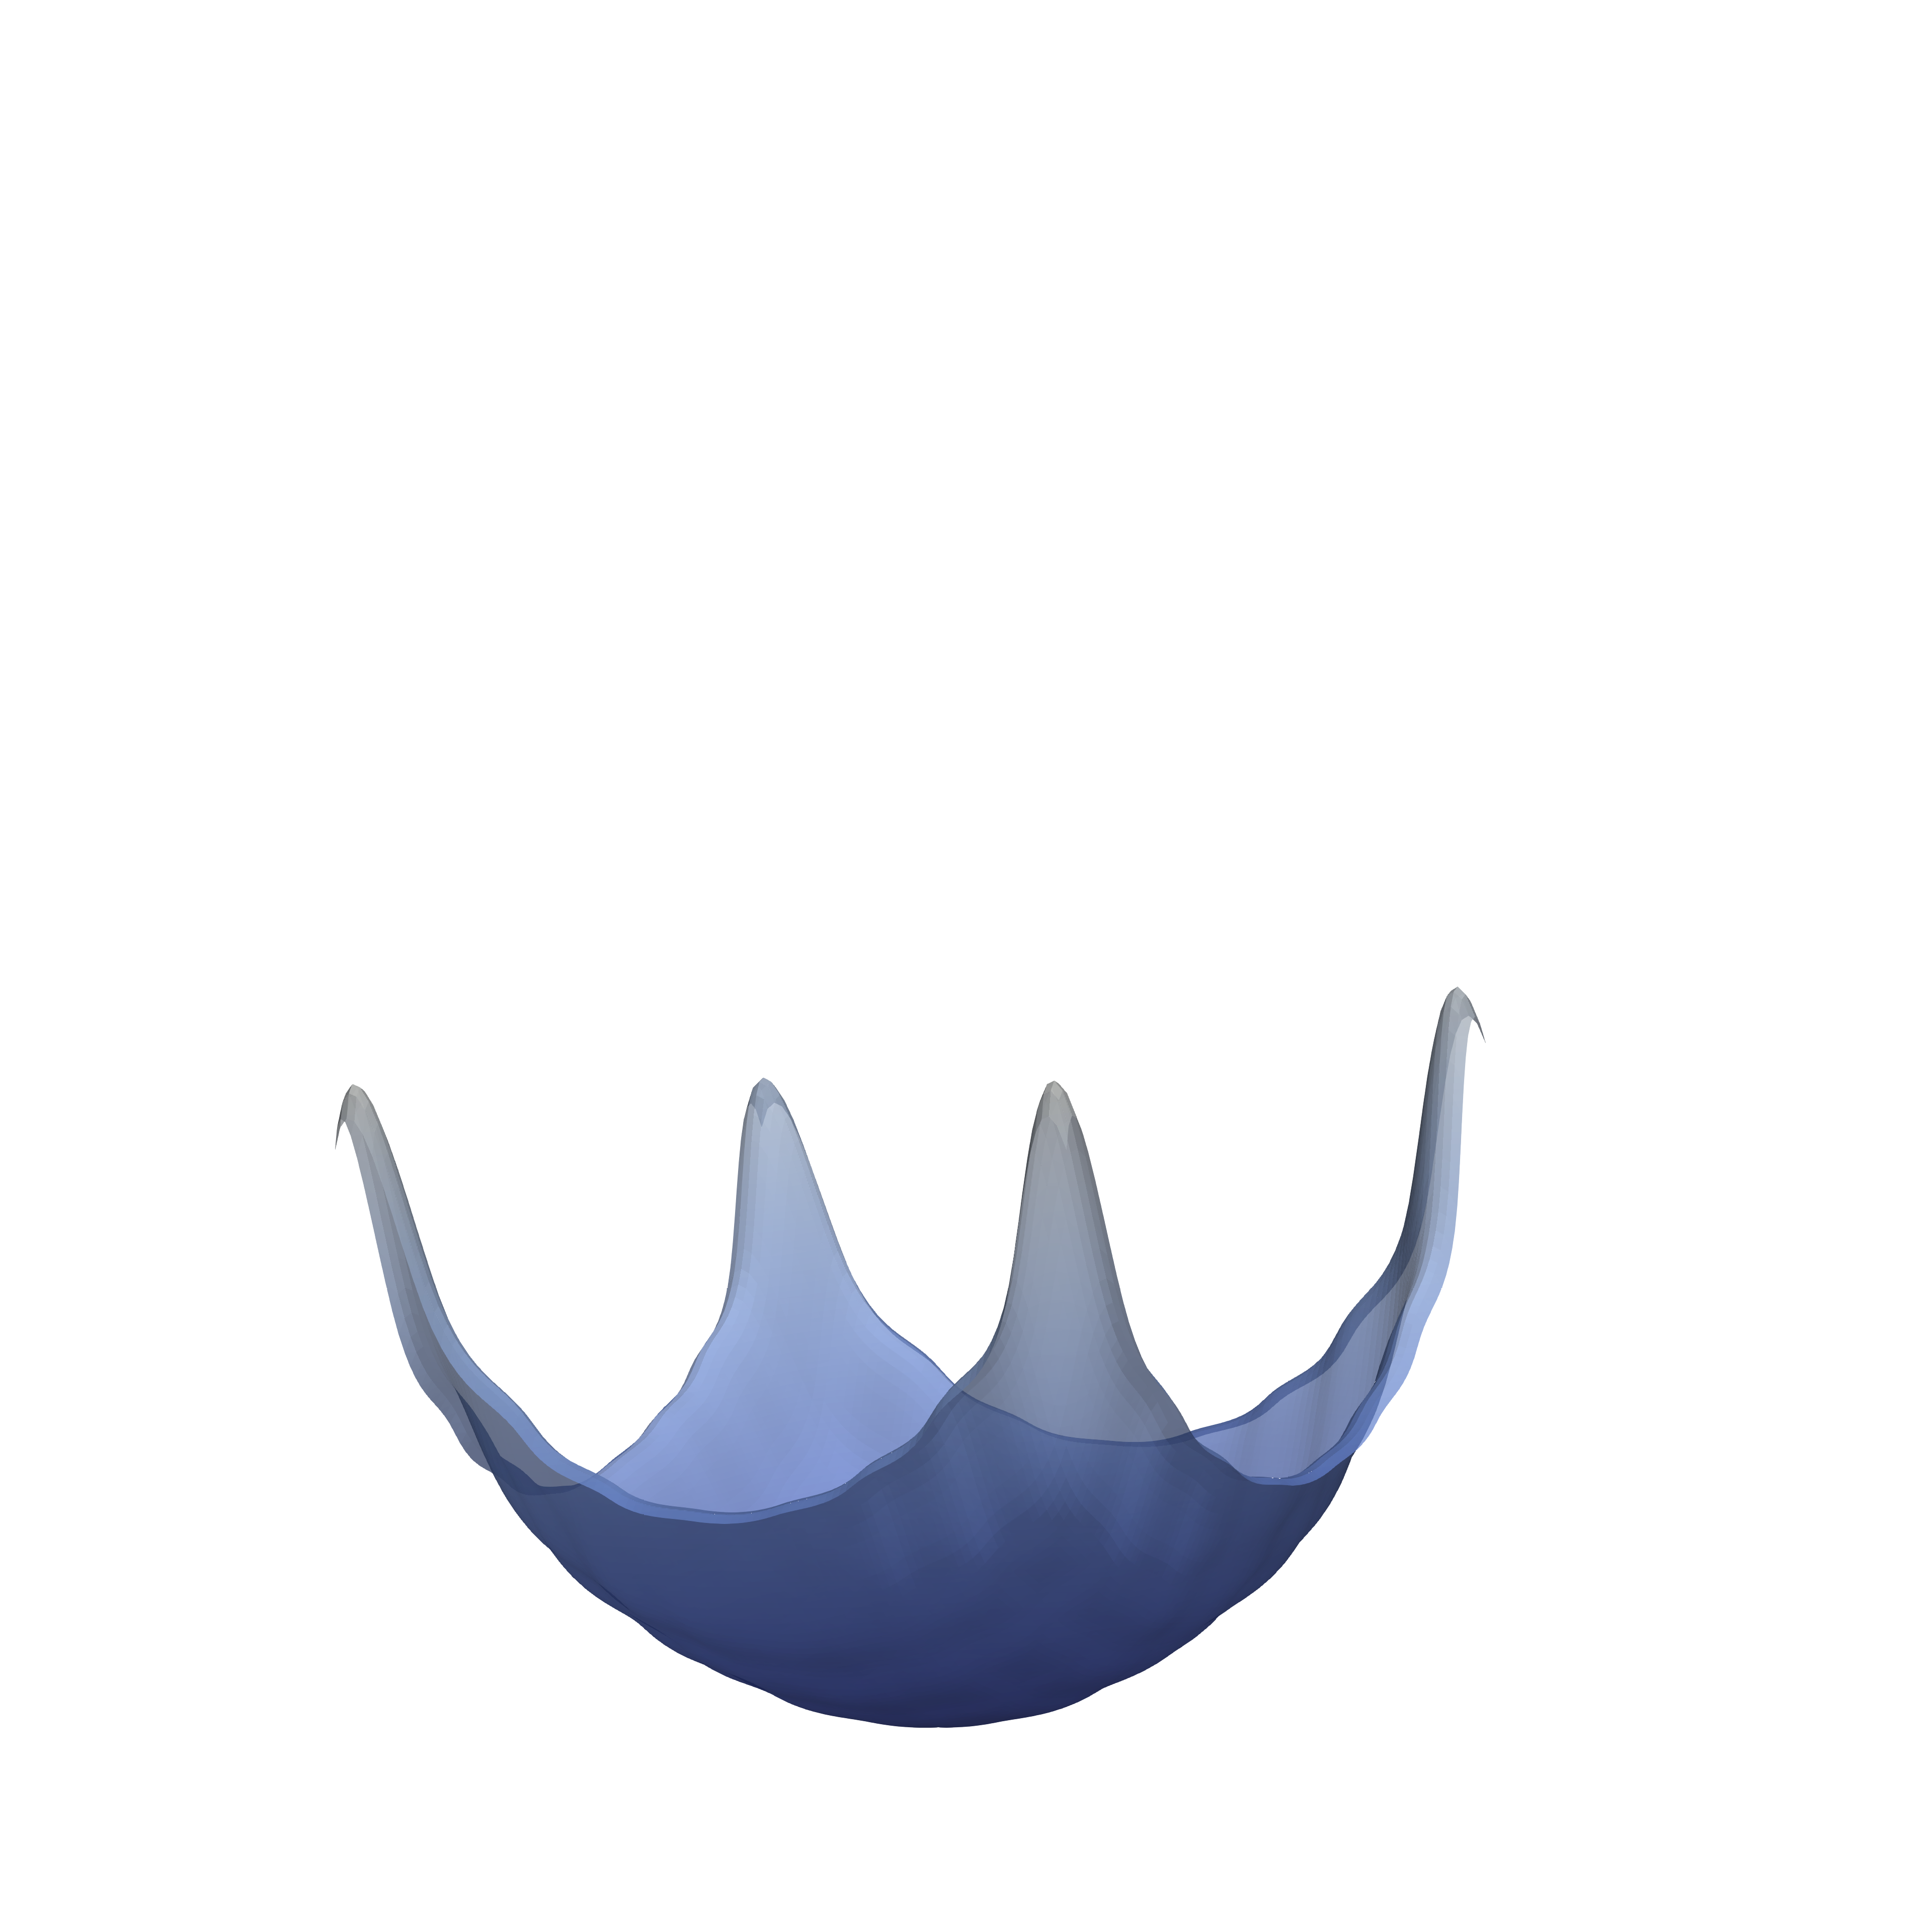}
    \caption{Model Width: 64}
    \label{fig:Transformer64}
\end{subfigure}
% Second row
\begin{subfigure}{0.23\textwidth}
    \includegraphics[width=\linewidth]{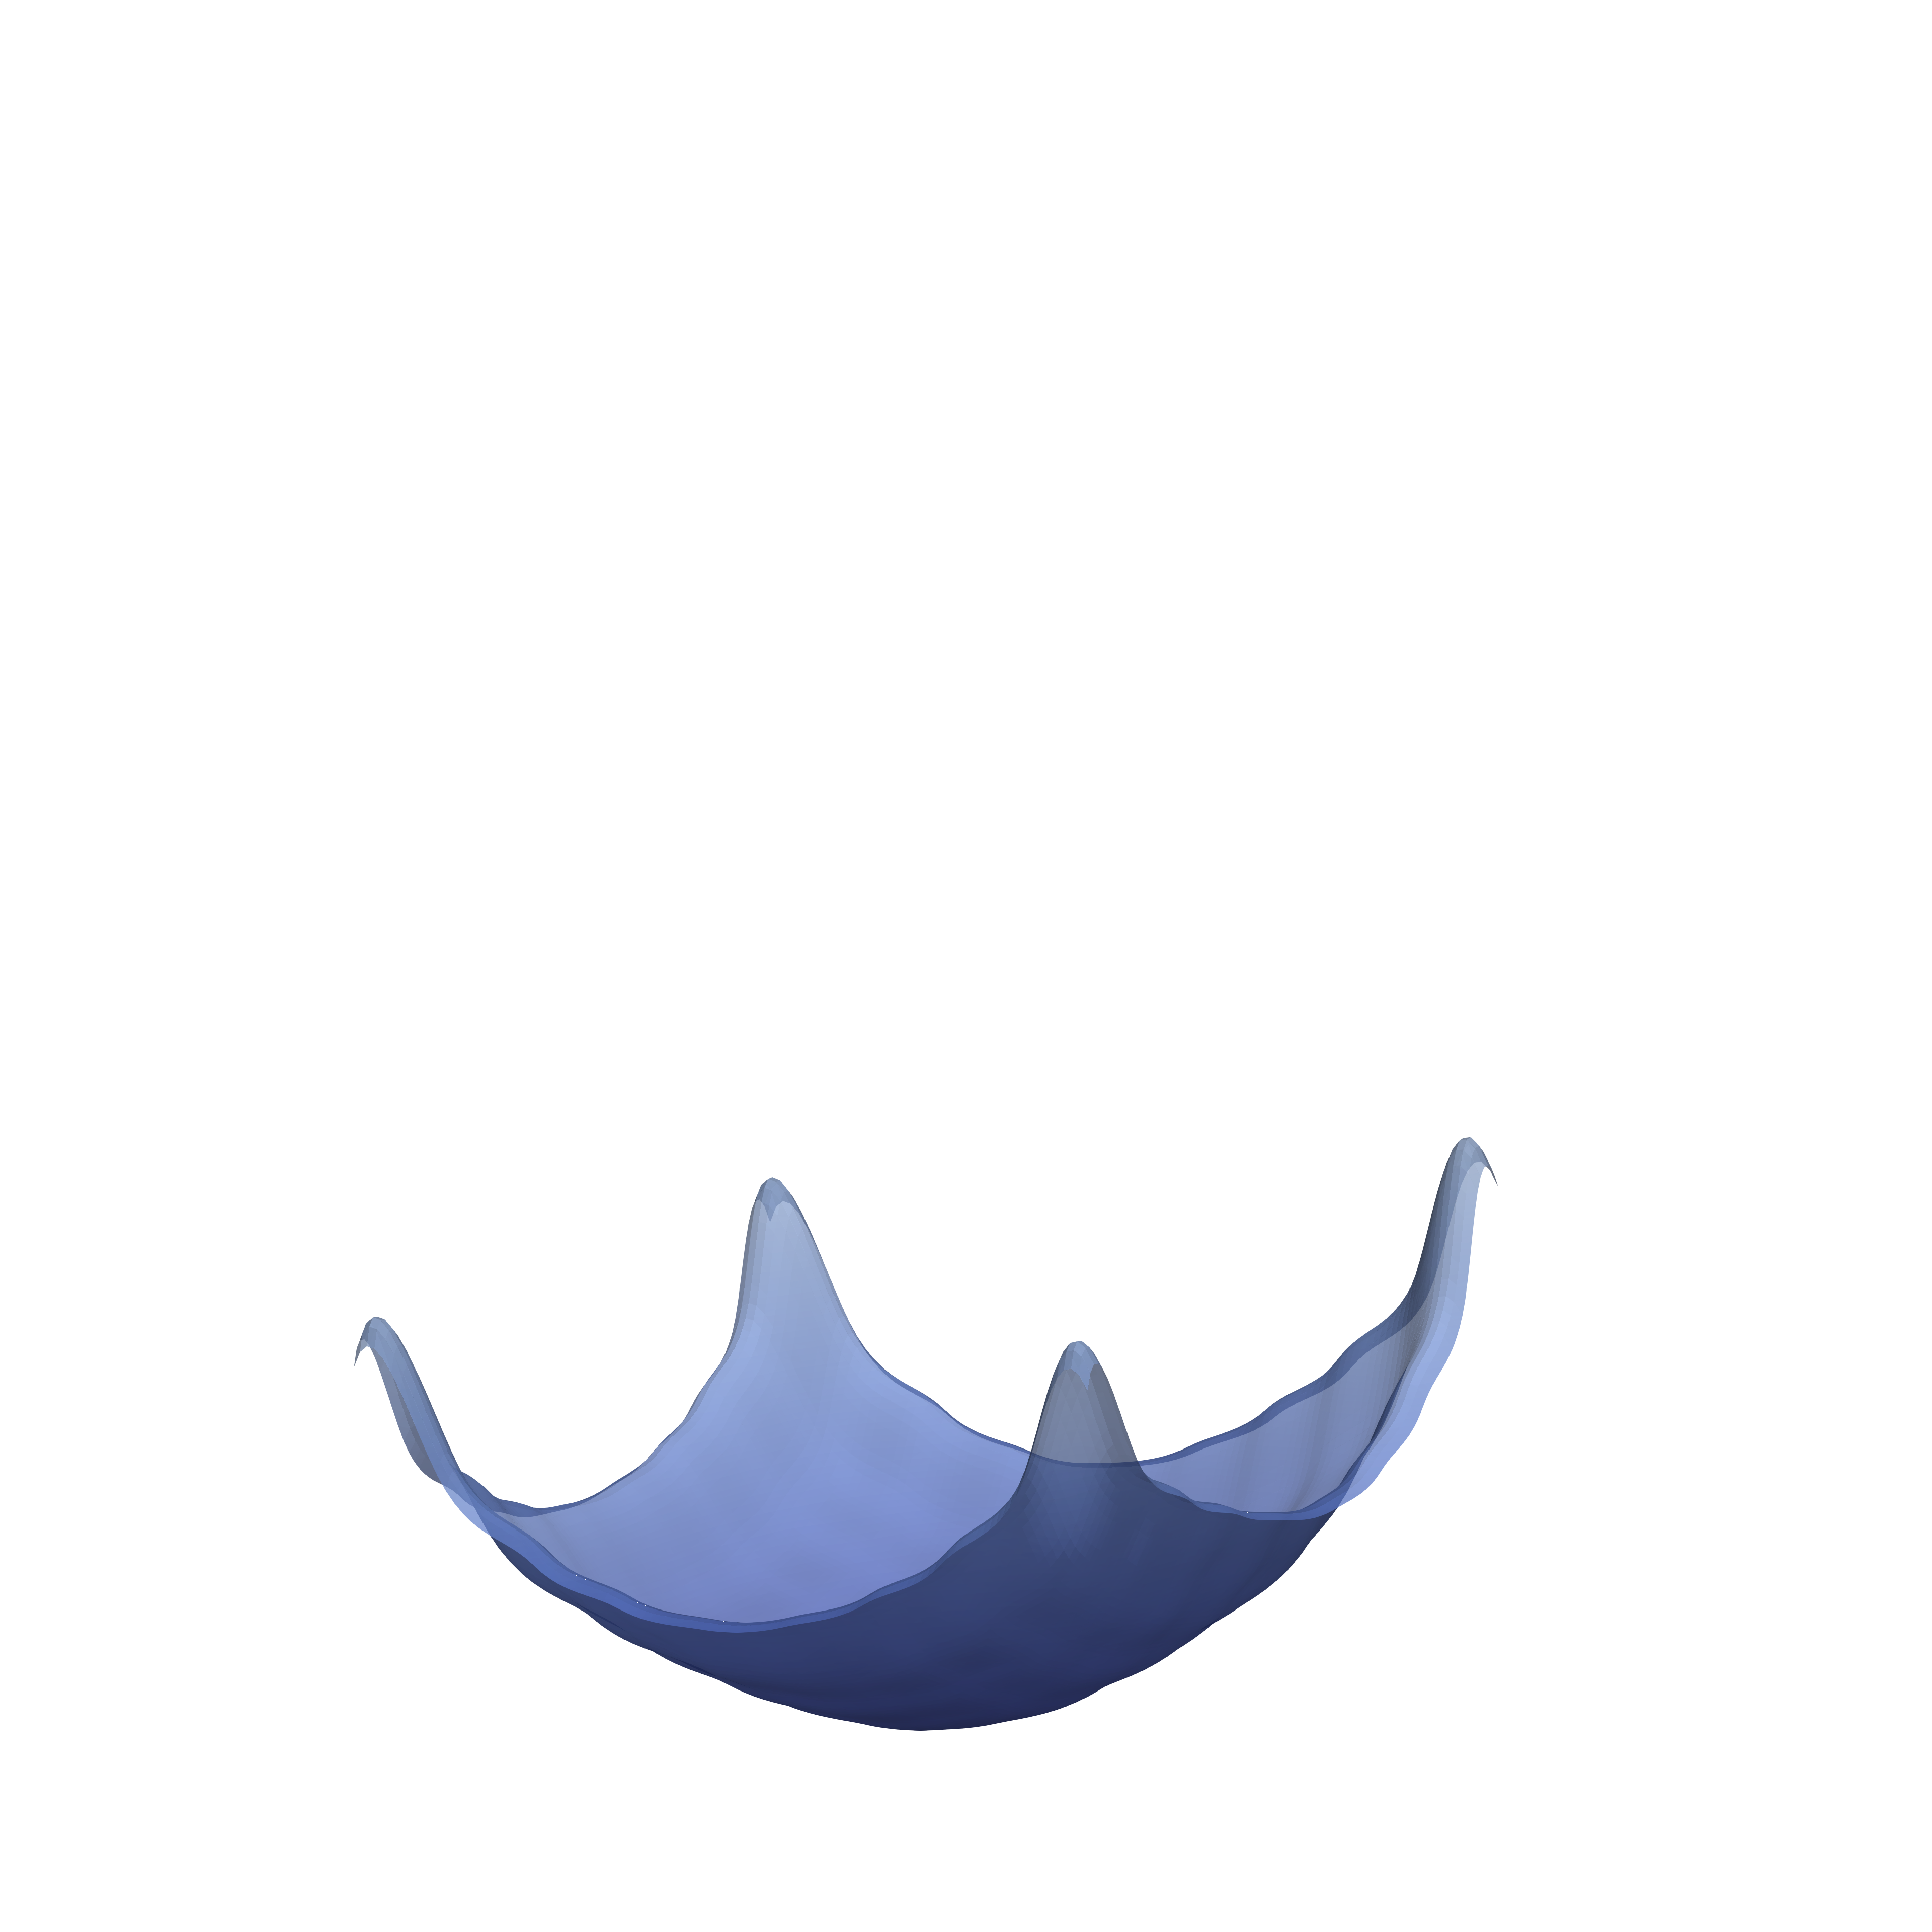}
    \caption{Model Width: 96}
    \label{fig:Transformer96}
\end{subfigure}
\begin{subfigure}{0.23\textwidth}
    \includegraphics[width=\linewidth]{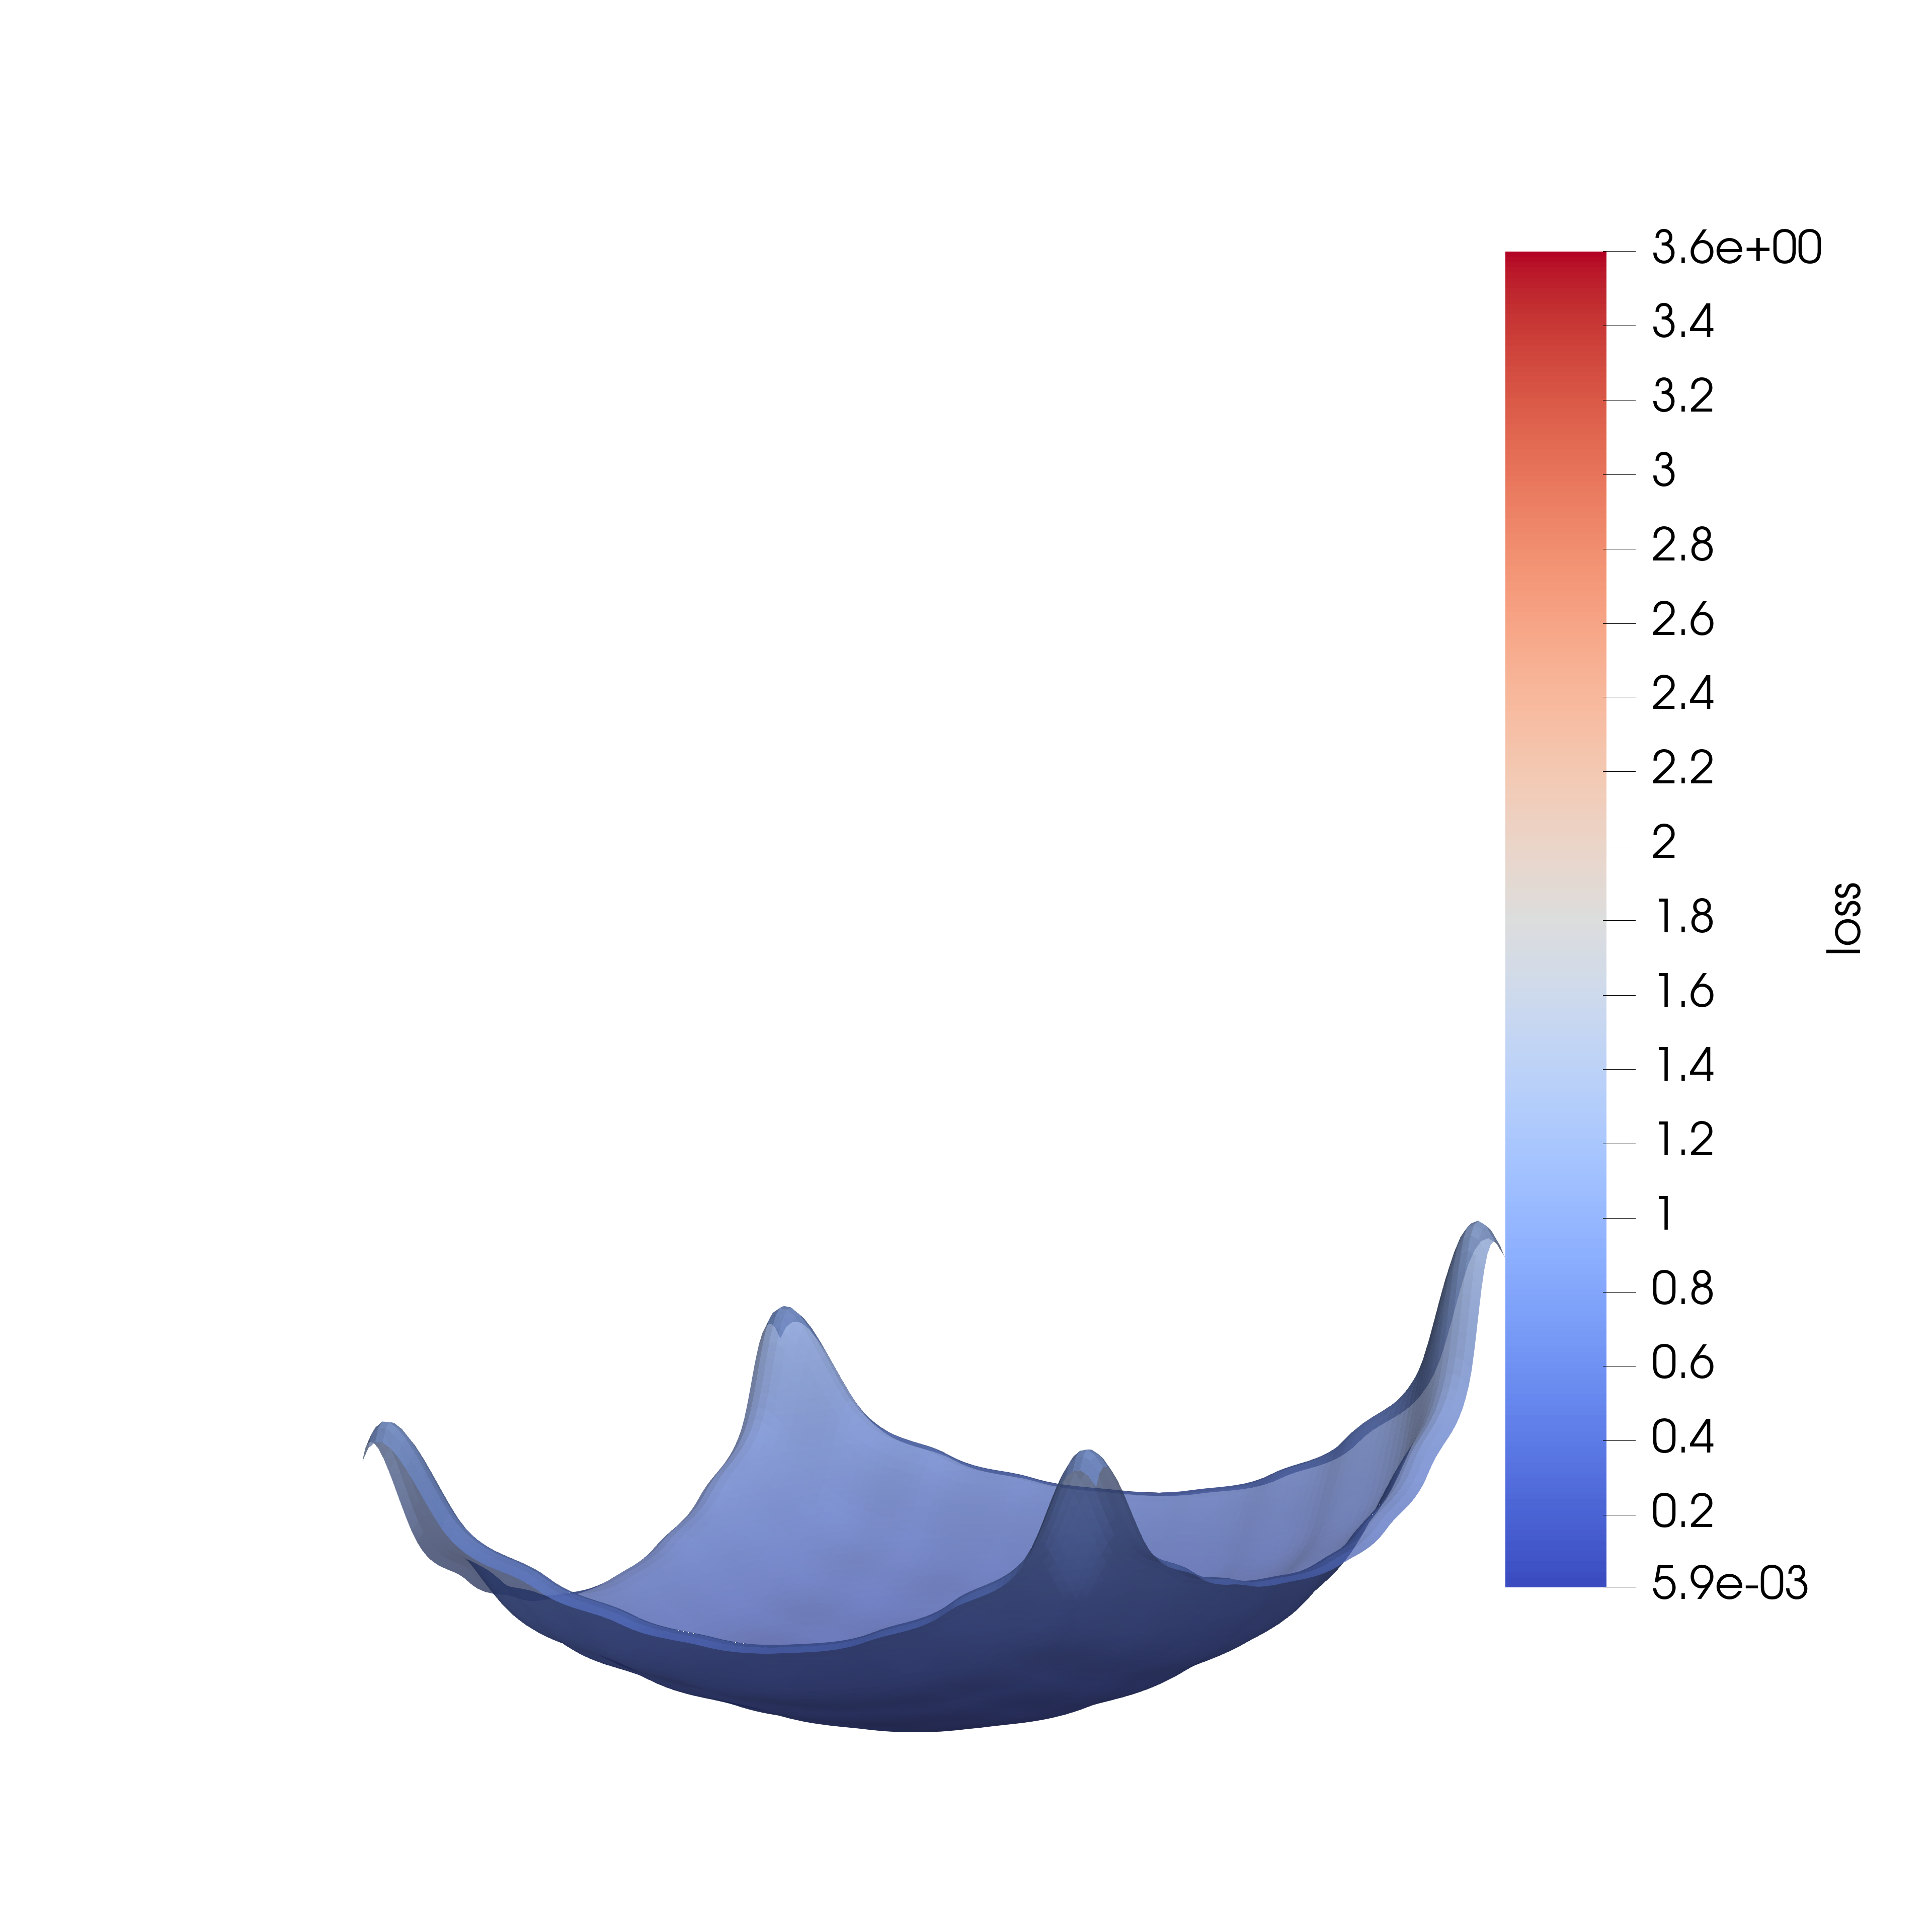}
    \caption{Model Width: 128}
    \label{fig:Transformer128}
\end{subfigure}

\caption{Effect of model width on loss landscape (Transformer Model)}
\label{fig:TransformerWidth}
\end{figure}

\begin{figure}[ht]
\centering
% First row
\begin{subfigure}{0.23\textwidth}
    \includegraphics[width=\linewidth]{figures/stu_ll/32.png}
    \caption{Model Width: 32}
    \label{fig:STU32}
\end{subfigure}
\begin{subfigure}{0.23\textwidth}
    \includegraphics[width=\linewidth]{figures/stu_ll/64.png}
    \caption{Model Width: 64}
    \label{fig:STU64}
\end{subfigure}
% Second row
\begin{subfigure}{0.23\textwidth}
    \includegraphics[width=\linewidth]{figures/stu_ll/96.png}
    \caption{Model Width: 96}
    \label{fig:STU96}
\end{subfigure}
\begin{subfigure}{0.23\textwidth}
    \includegraphics[width=\linewidth]{figures/stu_ll/128.png}
    \caption{Model Width: 128}
    \label{fig:STU128}
\end{subfigure}

\caption{Effect of model width on loss landscape (STU Model).}
\label{fig:STUWidth}
\end{figure}

\begin{figure}[ht]
\centering
% First row
\begin{subfigure}{0.23\textwidth}
    \includegraphics[width=\linewidth]{figures/stuT_ll/32.png}
    \caption{Model Width: 32.}
    \label{fig:STUT32}
\end{subfigure}
\begin{subfigure}{0.23\textwidth}
    \includegraphics[width=\linewidth]{figures/stuT_ll/64.png}
    \caption{Model Width: 64.}
    \label{fig:STUT64}
\end{subfigure}
% Second row
\begin{subfigure}{0.23\textwidth}
    \includegraphics[width=\linewidth]{figures/stuT_ll/96.png}
    \caption{Model Width: 96.}
    \label{fig:STUT96}
\end{subfigure}
\begin{subfigure}{0.23\textwidth}
    \includegraphics[width=\linewidth]{figures/stuT_ll/128.png}
    \caption{Model Width: 128.}
    \label{fig:STUT128}
\end{subfigure}

\caption{Effect of model width on loss landscape (STU-T Model).}
\label{fig:STUTWidth}
\end{figure}

\begin{figure}[ht]
\centering
% First row
\begin{subfigure}{0.23\textwidth}
    \includegraphics[width=\linewidth]{figures/hybrid_ll/32.png}
    \caption{Model Width: 32.}
    \label{fig:Hybrid32}
\end{subfigure}
\begin{subfigure}{0.23\textwidth}
    \includegraphics[width=\linewidth]{figures/hybrid_ll/64.png}
    \caption{Model Width: 64.}
    \label{fig:Hybrid64}
\end{subfigure}
% Second row
\begin{subfigure}{0.23\textwidth}
    \includegraphics[width=\linewidth]{figures/hybrid_ll/96.png}
    \caption{Model Width: 96.}
    \label{fig:Hybrid96}
\end{subfigure}
\begin{subfigure}{0.23\textwidth}
    \includegraphics[width=\linewidth]{figures/hybrid_ll/128.png}
    \caption{Model Width: 128.}
    \label{fig:Hybrid128}
\end{subfigure}

\caption{Effect of model width on loss landscape (Hybrid Model).}
\label{fig:HybridWidth}
\end{figure}

\begin{figure}[ht]
\centering
% First row
\begin{subfigure}{0.23\textwidth}
    \includegraphics[width=\linewidth]{figures/hybridT_ll/32.png}
    \caption{Model Width: 32.}
    \label{fig:HybridT32}
\end{subfigure}
\begin{subfigure}{0.23\textwidth}
    \includegraphics[width=\linewidth]{figures/hybridT_ll/64.png}
    \caption{Model Width: 64.}
    \label{fig:HybridT64}
\end{subfigure}
% Second row
\begin{subfigure}{0.23\textwidth}
    \includegraphics[width=\linewidth]{figures/hybridT_ll/96.png}
    \caption{Model Width: 96.}
    \label{fig:HybridT96}
\end{subfigure}
\begin{subfigure}{0.23\textwidth}
    \includegraphics[width=\linewidth]{figures/hybridT_ll/128.png}
    \caption{Model Width: 128.}
    \label{fig:HybridT128}
\end{subfigure}
\caption{Effect of model width on loss landscape (Hybrid-T Model).}
\label{fig:HybridTWidth}
\end{figure}

\begin{figure}[ht]
\centering
% First row
\begin{subfigure}{0.32\textwidth}
    \includegraphics[width=\linewidth]{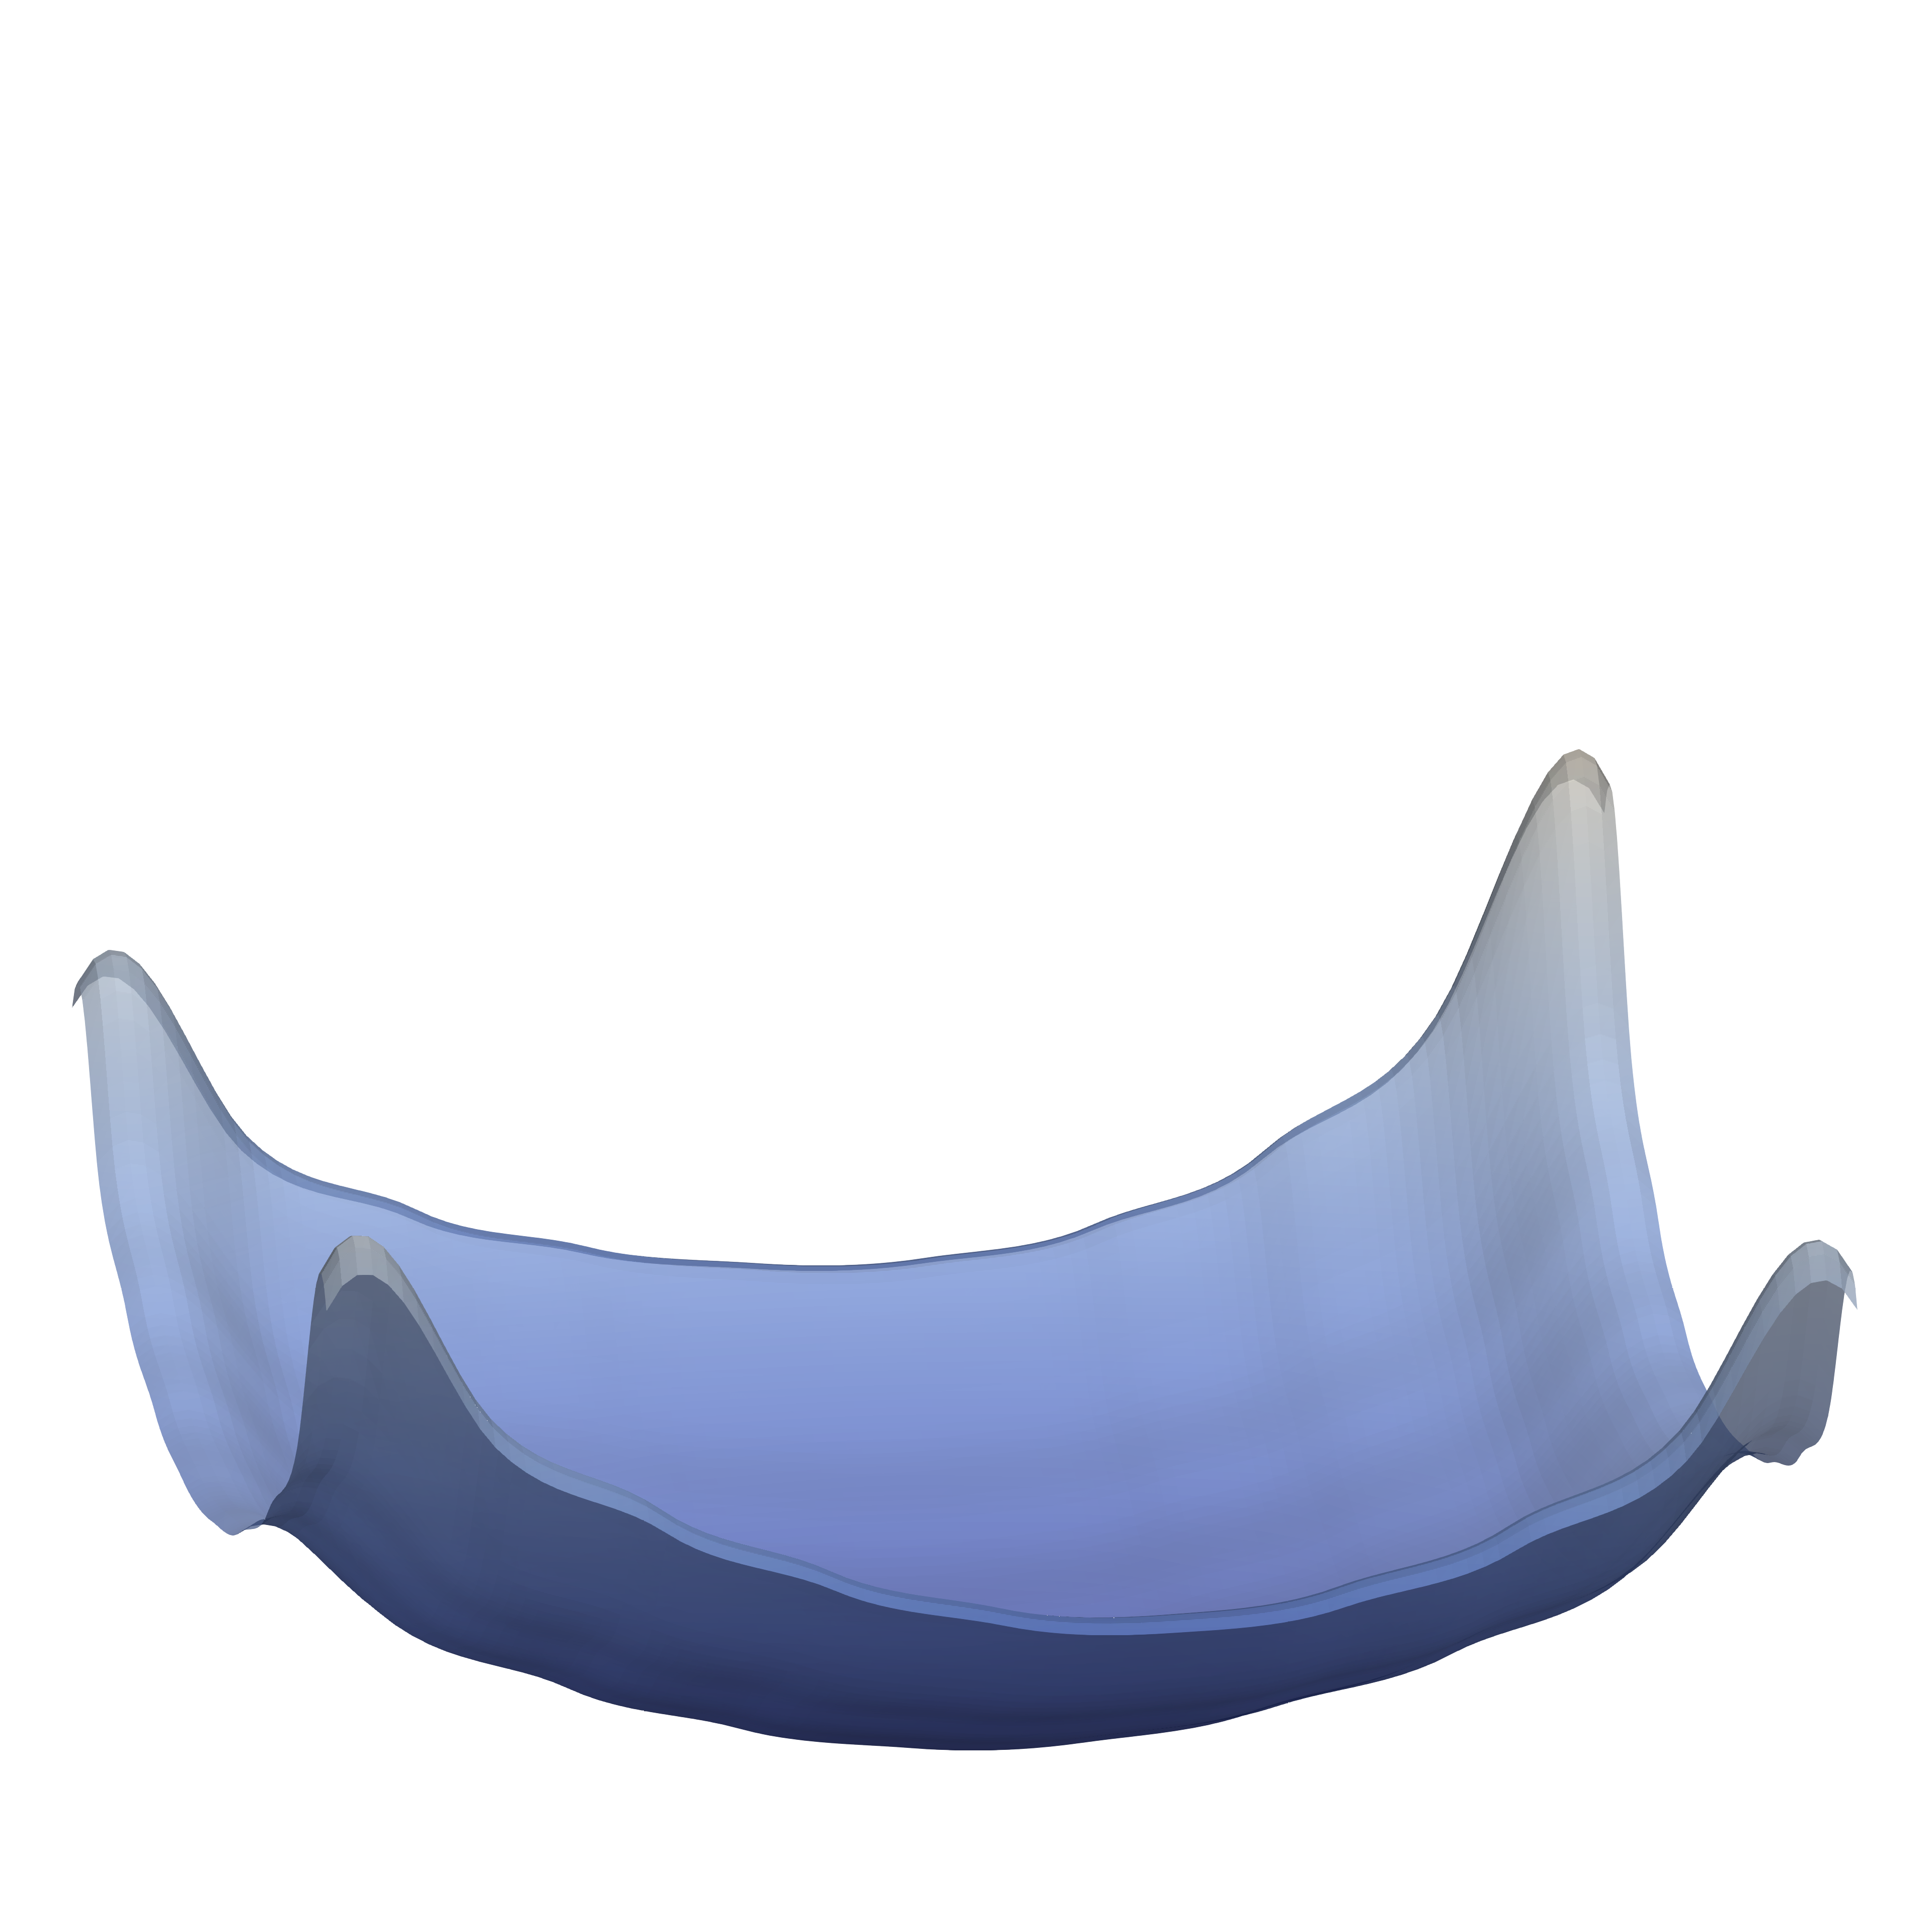}
    \caption{Transformer Model.}
    \label{fig:TransformerLL}
\end{subfigure}
\hfill
\begin{subfigure}{0.32\textwidth}
    \includegraphics[width=\linewidth]{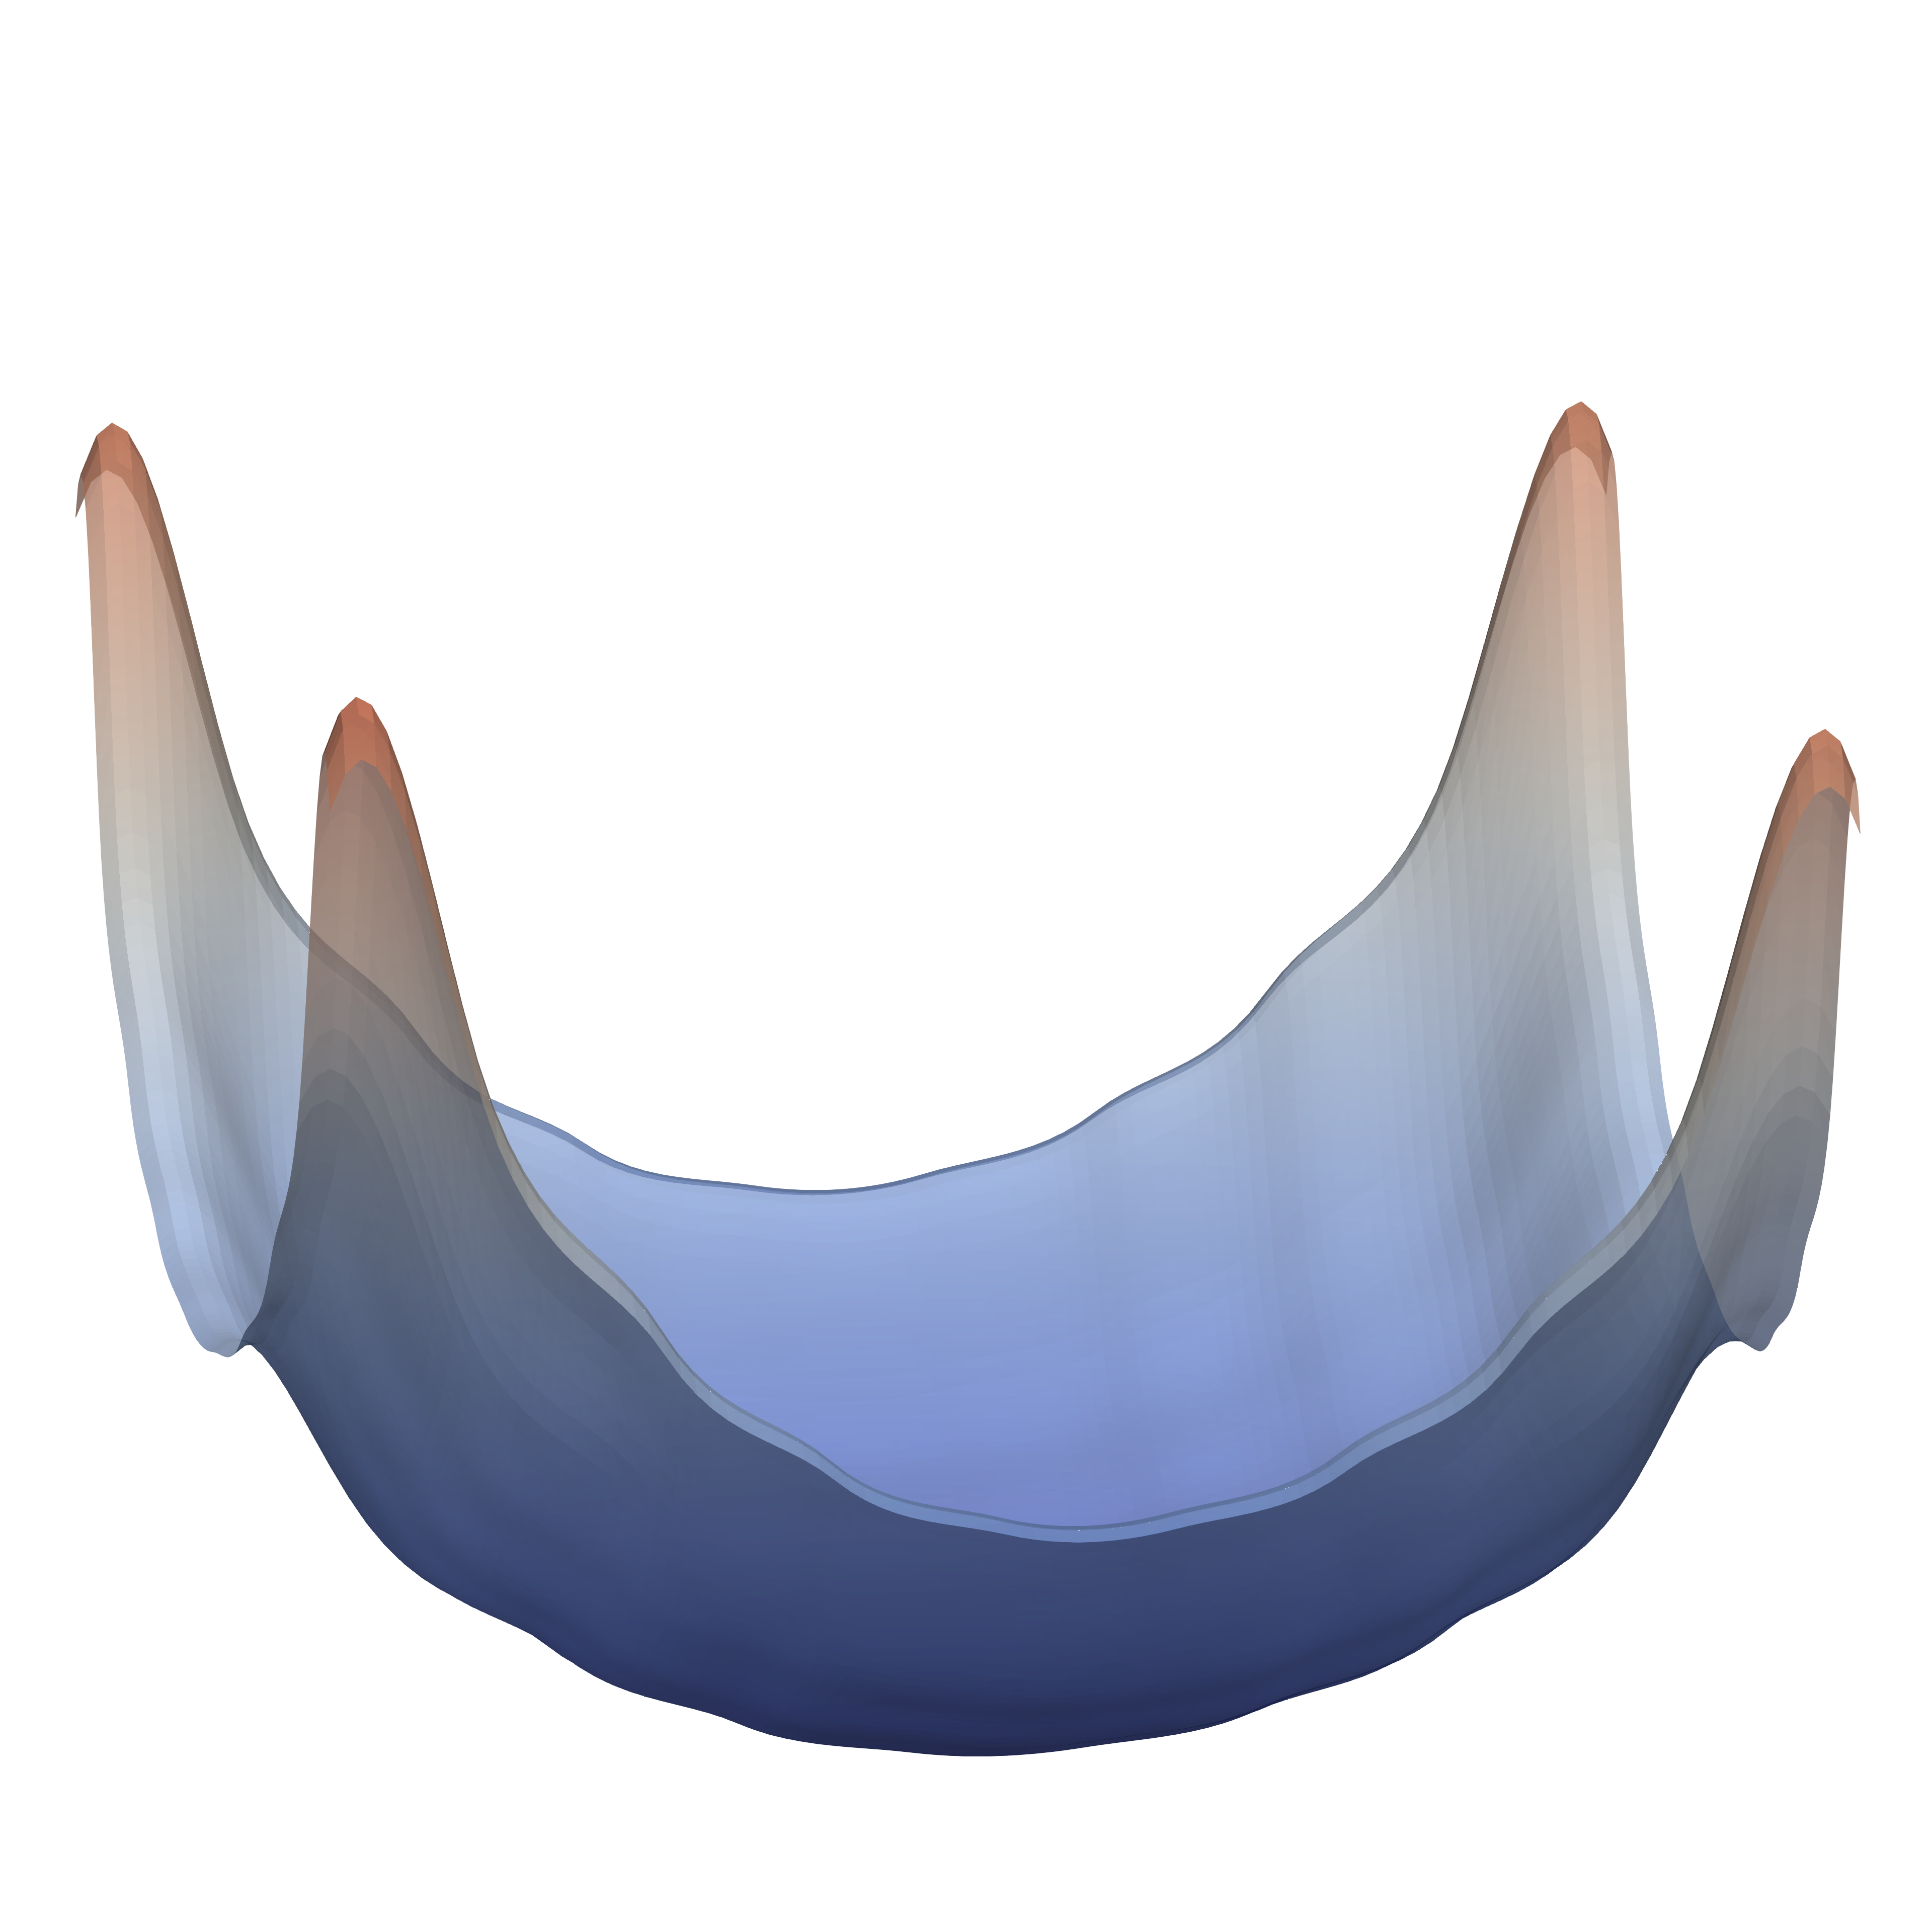}
    \caption{STU-Attention Hybrid.}
    \label{fig:HybridLL}
\end{subfigure}
\hfill
\begin{subfigure}{0.32\textwidth}
    \includegraphics[width=\linewidth]{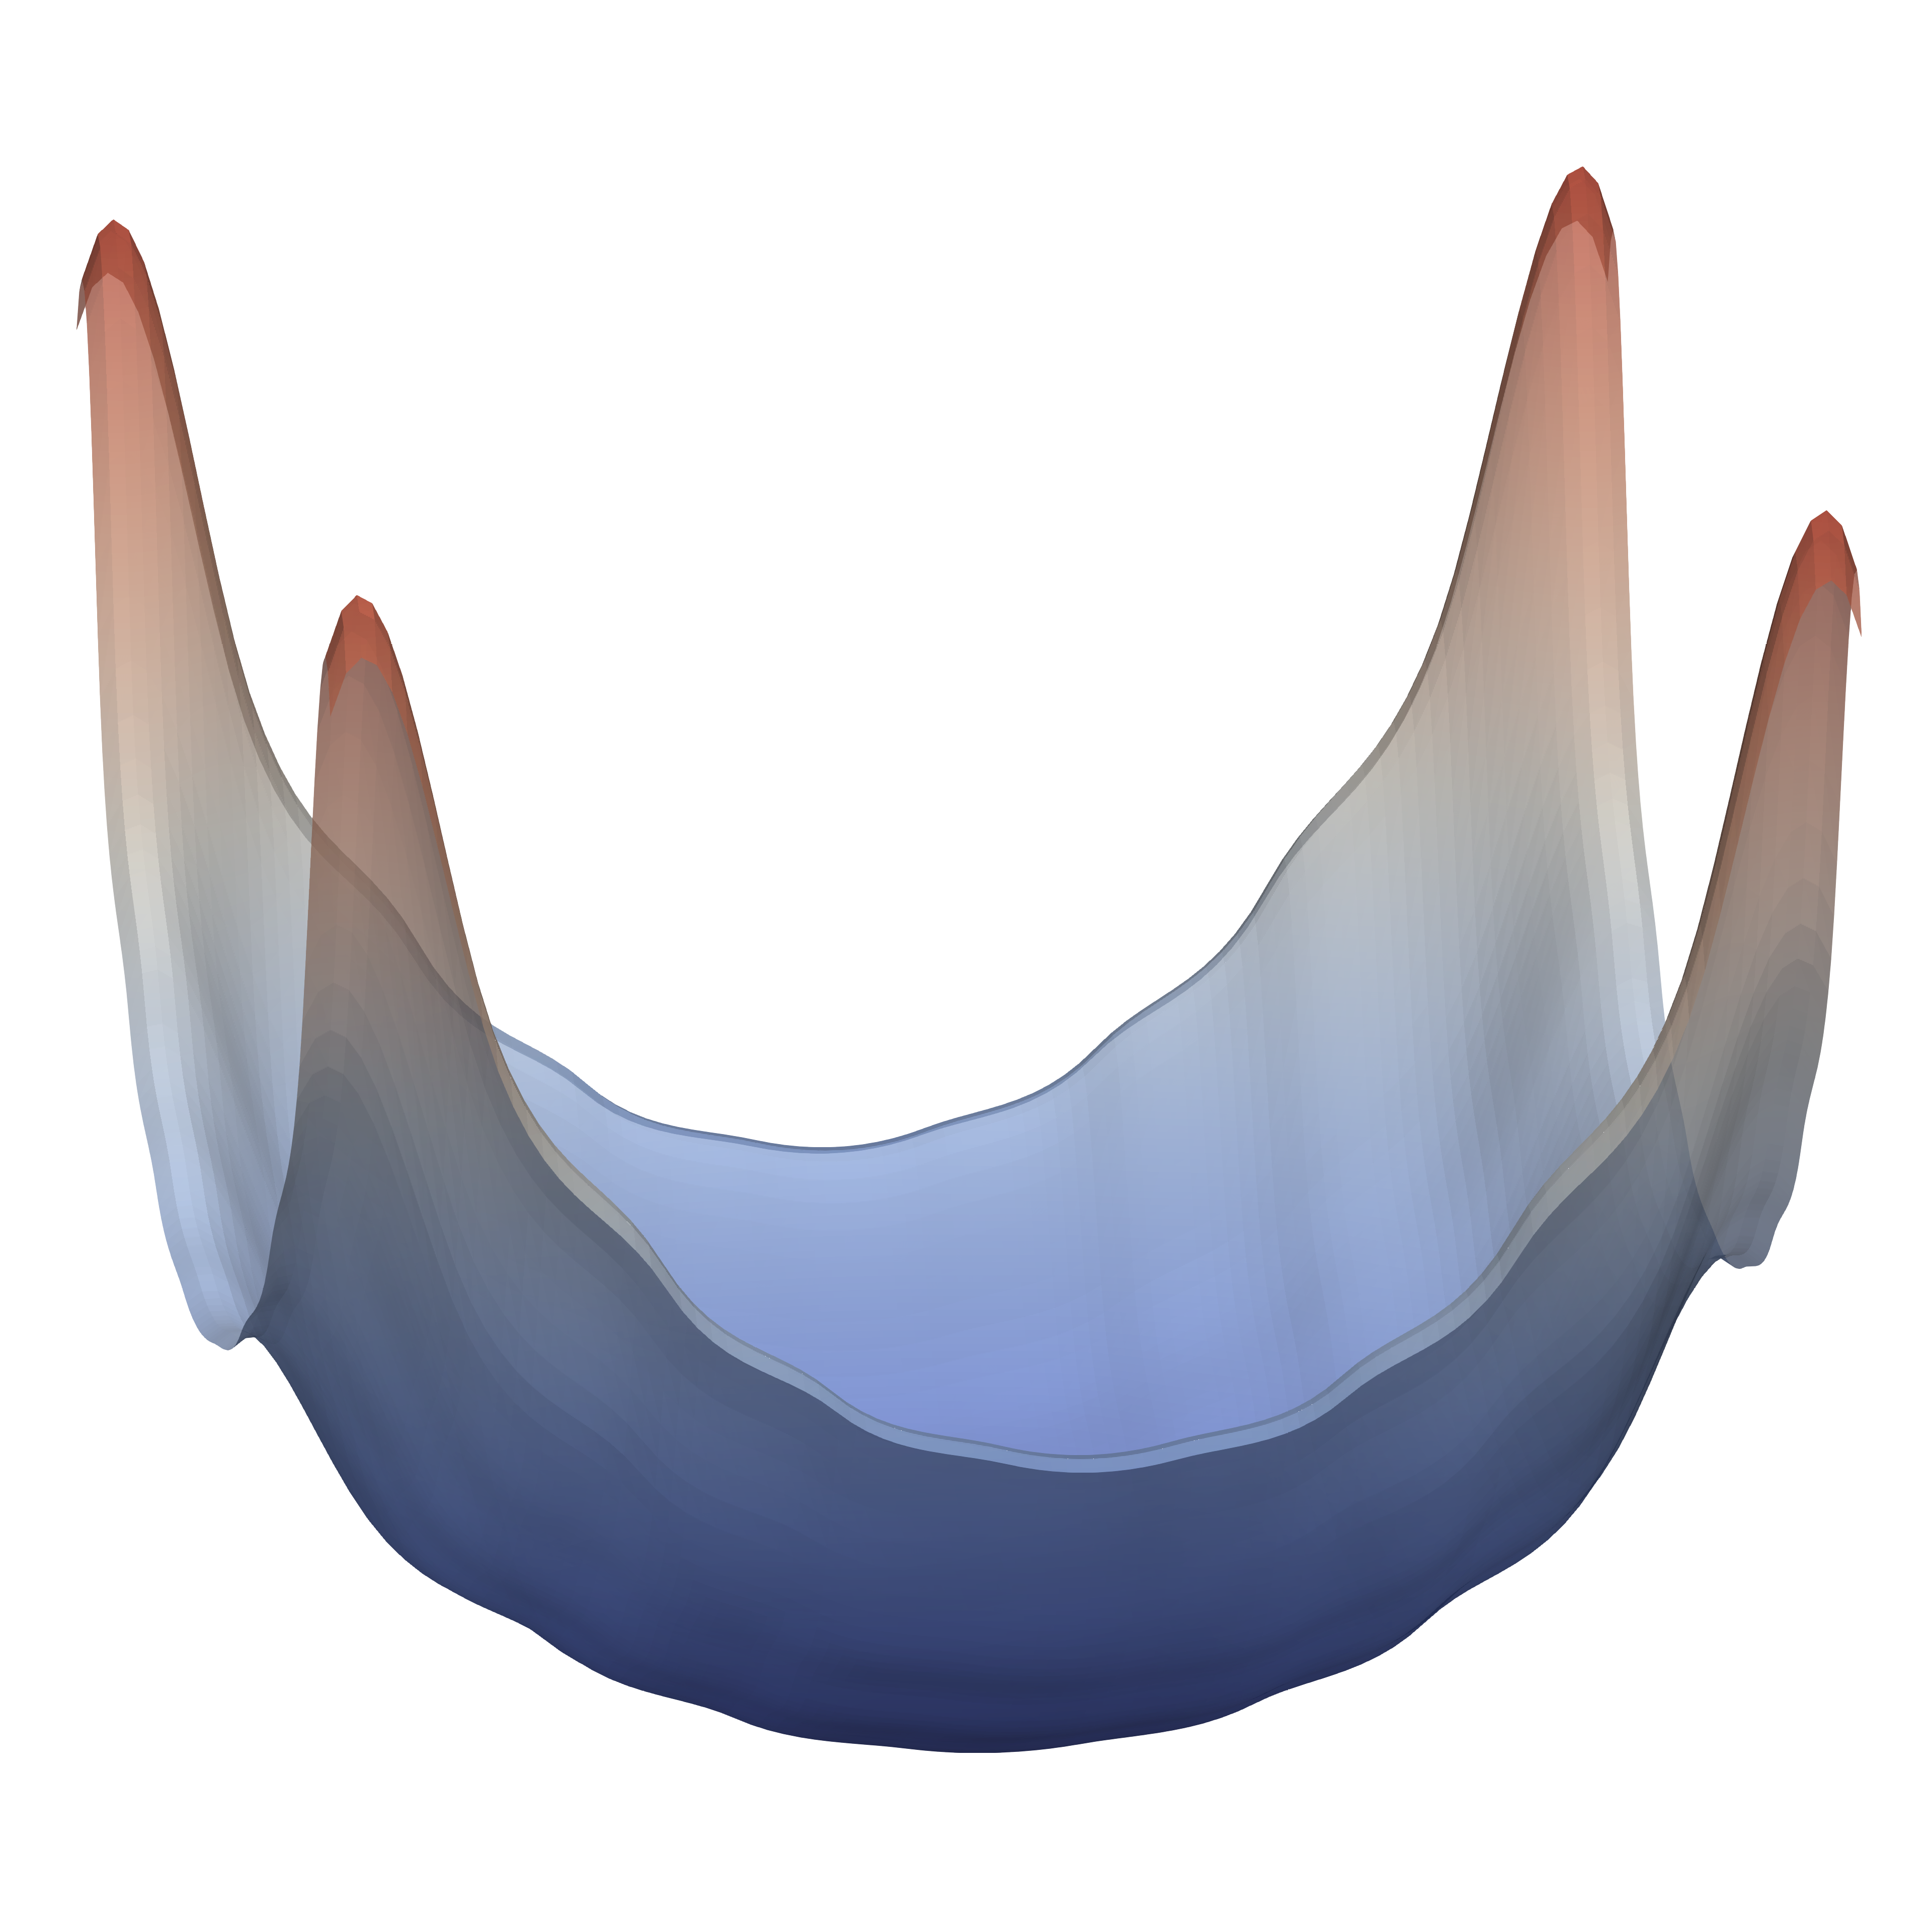}
    \caption{STU-T-Attention Hybrid.}
    \label{fig:HybridTLL}
\end{subfigure}
\vspace{2em}
\hspace{0.055\textwidth}
\begin{subfigure}{0.32\textwidth}
    \includegraphics[width=\linewidth]{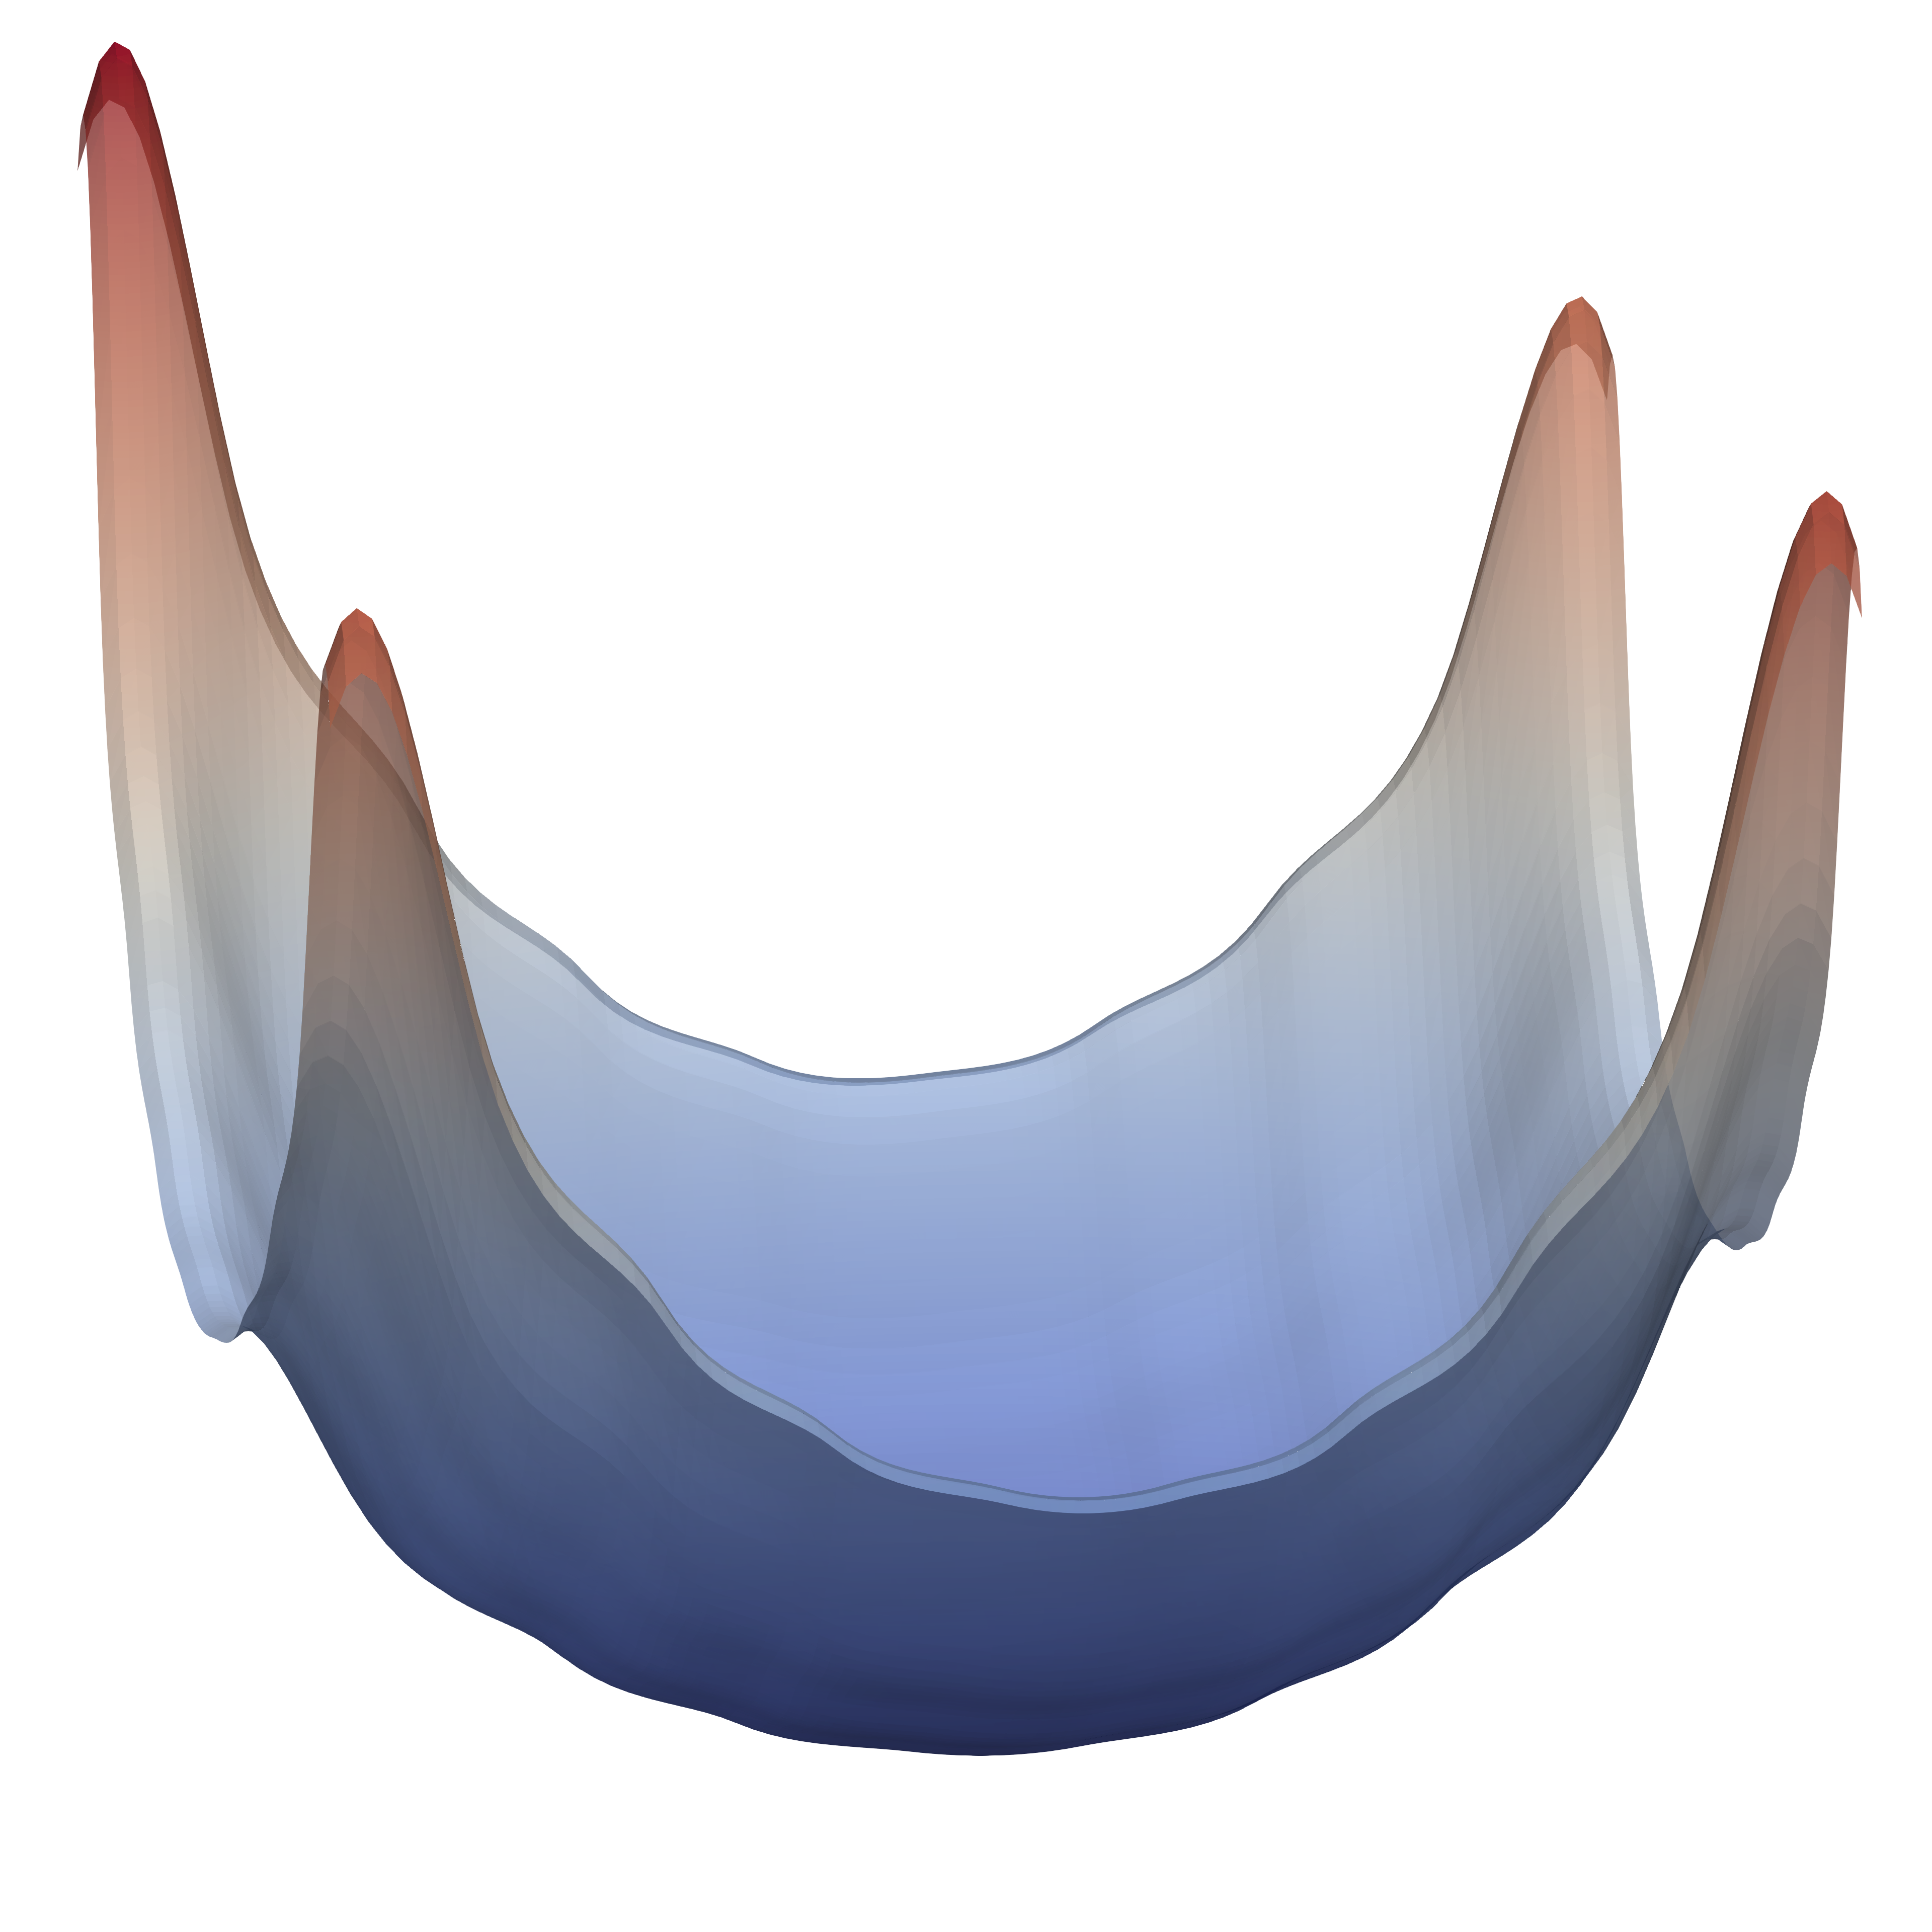}
    \caption{STU Model.}
    \label{fig:STULL}
\end{subfigure}
\hspace{1em}
\begin{subfigure}{0.32\textwidth}
    \includegraphics[width=\linewidth]{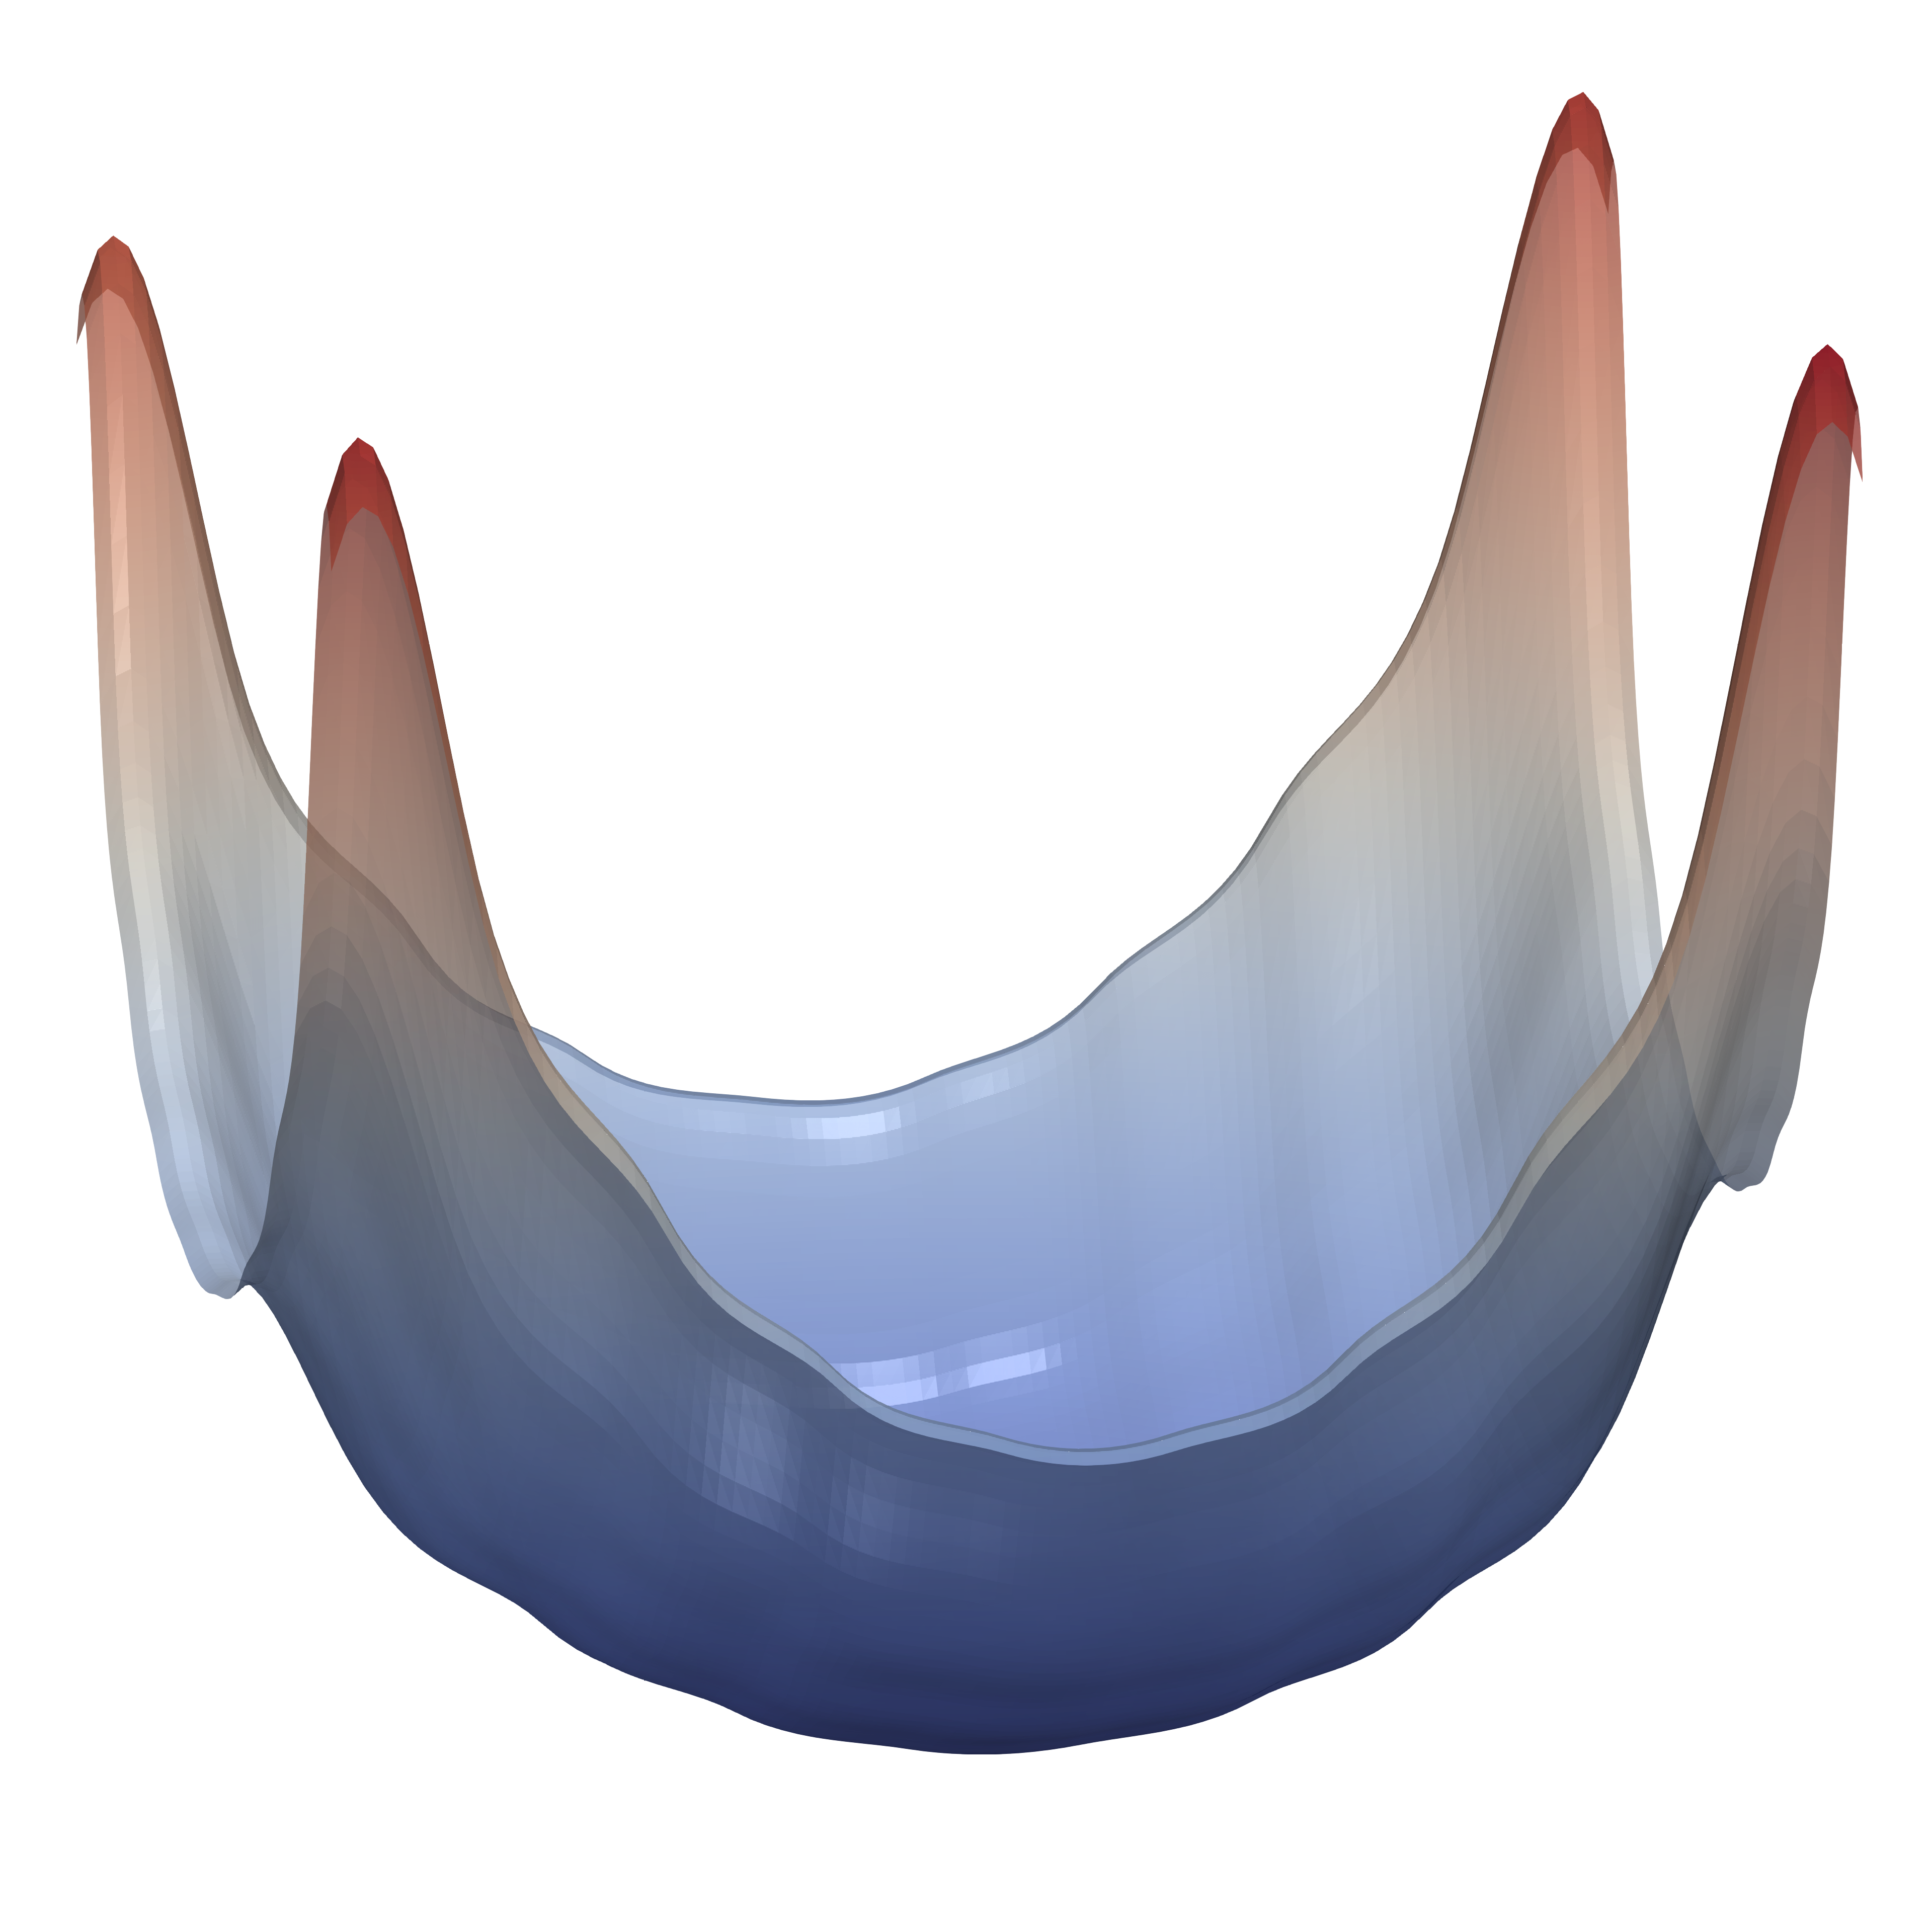}
    \caption{STU-T Model.}
    \label{fig:STUTLL}
\end{subfigure}
\begin{subfigure}{0.055\textwidth}
    \includegraphics[width=\linewidth]{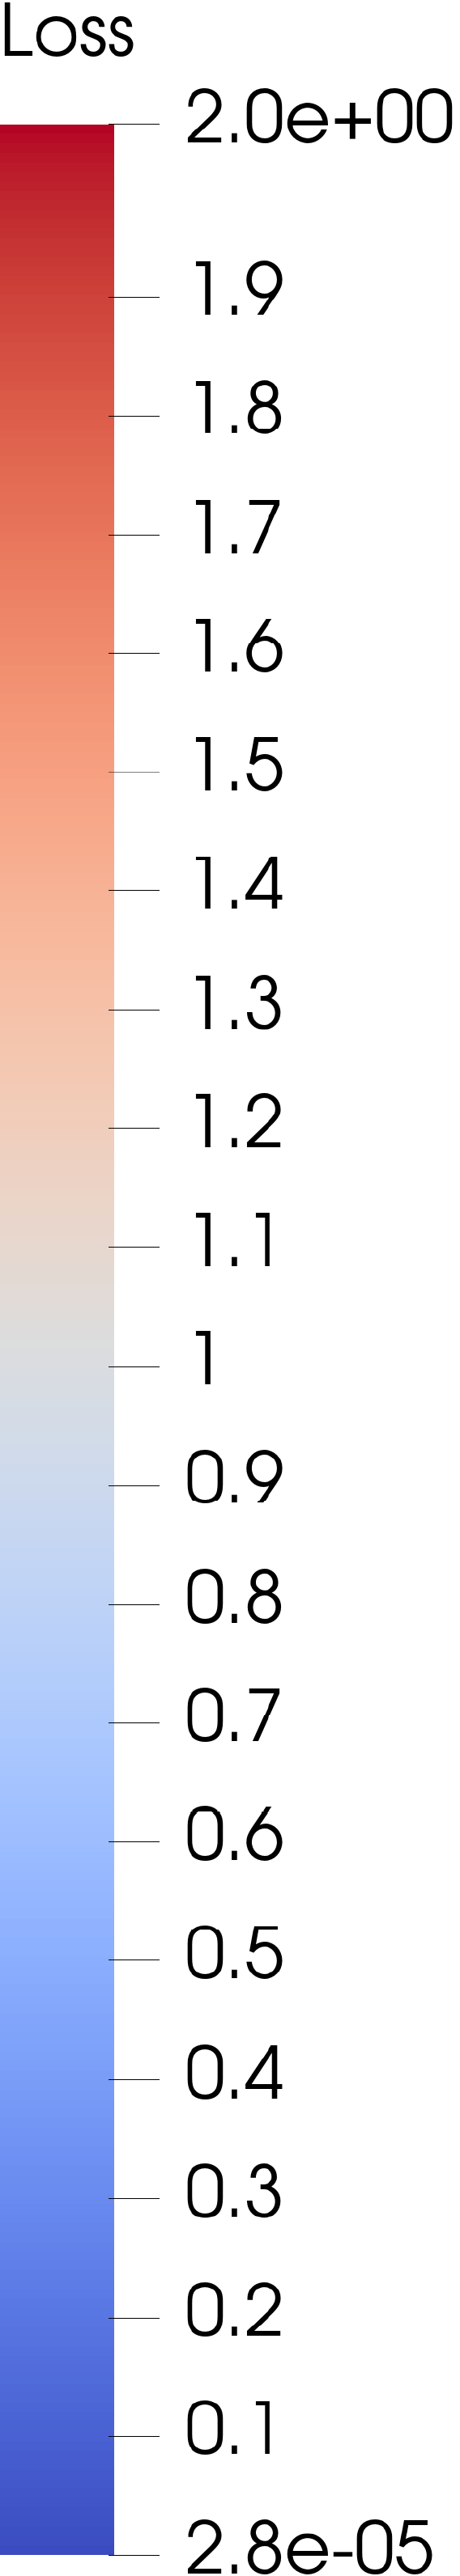}
    \caption*{}
    \label{fig:cbar2}
\end{subfigure}
\caption{Loss landscapes for models with 4 layers and model width 128.}
\label{fig:Models-LL}
\end{figure}
